# Supplementary material for: Aligned Multi Objective Optimization
Source: arXiv:2502.14096 source file (2025-03-04)
Supplement: Supplementary file 1 [file appendix.tex]

\begin{figure}[htbp]
\centering
\begin{minipage}{0.9\textwidth}
    \centering
    \includegraphics[width=1.0\textwidth]{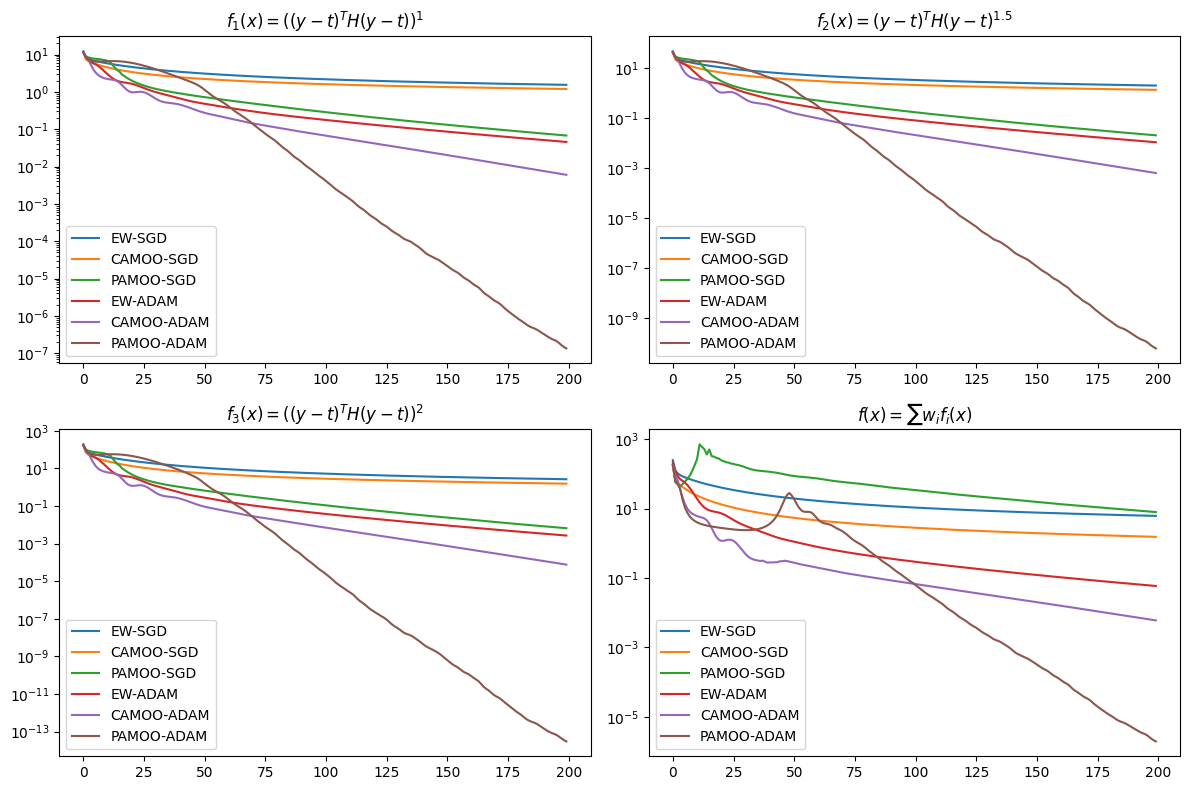}
    \caption{Local curvature example, all loss functions.}\label{fig:local_curvature_losses}
\end{minipage}

\vspace{1cm}

\begin{minipage}{0.9\textwidth}
    \centering
    \includegraphics[width=1.0\textwidth]{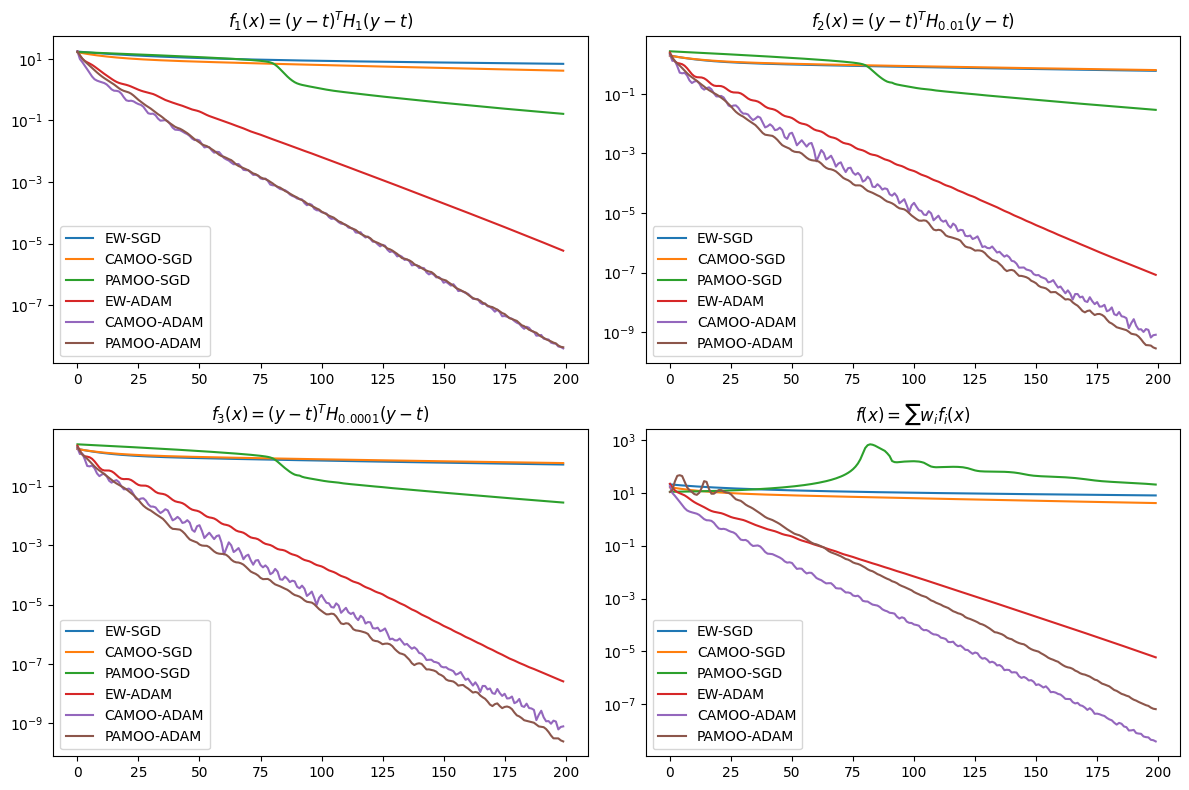}
    \caption{Selection example, all loss functions.}\label{fig:selection_losses}
\end{minipage}
\label{fig:subfigures}
\end{figure}

\section{Additional Experimental Details}\label{app:practical_implementation}

We share an IPython notebook in which we implement our algorithms and was used to generate all plots accompanies this submission.

\textbf{Dataset.}
We sample 200 points from an independent uniform distribution $\x_i\in \mathrm{Uniform}([-1,1]^{20})$. 
We generate target data from a randomly initialized network $t(x_i) = h_{\theta_\star}(x_i) + 10.$
The target dimension is $7$.

%
\textbf{Network architecture.}
We choose the ground truth network and target network to have the same architecture. Both are 2 layer neural networks with 512 hidden dimensions and ReLu activation. The neural network outputs a vector in dimension $7$.
%

\textbf{Training.}
For both problems, we set the learning rate of SGD to $0.0005$ and ADAM to $0.005$, we use the same learning rates for \PAMOO. For \CAMOO we multiply the learning rate by the number of loss functions, $3$. While equal weighting sets all weights to 1, \CAMOO is constrained to set the sum of all weights to one, our adjustment accounts for this normalization.
% We perform each run with 5 different seeds and average their performance.
%

% \textcolor{red}{YE: todo. we currently do not validation dataset so i removed this section.}

\textbf{General parameters for \CAMOO.}
We set the number of samples for the Hutchinson method to be $N_{\mathrm{Hutch}}=10$. Namley, we estimate the Hessian matrices by averaging $N_{\mathrm{Hutch}}=10$ estimates obtained from the Hutchnison method.  Further, at each training step we perform a single update of the weights based on the PU update rule of~\citet{cen2021fast} to solve the max-min Bilinear optimization problem (see Section~\ref{sec:prac_imp}). We use their primal-dual algorithm, and choose the learning rate as they specified $1 / (2 \max_{i,j}|\A_{ij}| + \tau_{\CAMOO})$ where $\A$ is the matrix in the Bilinear optimization problem and $\tau_{\CAMOO}=0.01$ is a regularization parameter we choose. Additionally, we set the number of iterations of the primal-dual algorithm to be $100$ per-step. We did not choose either parameter with great care, exploring best settings is part of future explorations.
%

\textbf{General parameters for \PAMOO.} We solved the constraint convex optimization problem in \PAMOO\ (see Algorithm~\ref{alg:PAMOO}) via the projected GD algorithm, where the projection on $\mathbb{R}^m_+$ is done by clipping negative values to $10^{-6}$. We set the learning rate to be $3e^{-3}$, and added a small regularization $\J_\x^\top\J_\x \rightarrow \J_\x^\top\J_\x + \tau_{\PAMOO} \I$ to avoid exploding weights, where $\tau_{\PAMOO}=1e^{-4}.$ 
% We performed 1000 gradient steps.


\textbf{Additional Plots.}
% We measure the $L_2$ distance between $h_\theta$ and $h_{\theta_\star}$ averaged over $1024\cdot10^3$ validation points and measured per dimension. This quantity suppose to approximate the quality of the learned model $\theta$ which is given by $\mathbb{E}_{x}\left[\enorm{h_\theta(\x)-h_{\theta_\star}(\x)}^2\right]$.
For completeness, we present the three loss functions of the objectives $\{ f_i \}_{i\in [3]}$ and the weighted loss as a function of GD iterates. Figure~\ref{fig:local_curvature_losses} depicts the losses for the local curvature example instance, and Figure~\ref{fig:selection_losses} depicts the losses for the selection example instance. Unlike \texttt{EW}, \CAMOO\ and \PAMOO\ adaptively modify the weight vector and adjust it to current parameters. 

We measured the weight vector as a function of GD iterates and present the results in Figure~\ref{fig:app_weight_vector_evolution}. 
\begin{itemize}
    \item \textbf{Local curvature example instance.} For the local curvature example instance we expect to see a switching behavior in \CAMOO\ (see Figure~\ref{fig:camoo_local}). Namely, when the loss is large, the weight vector of \CAMOO\ should assign most of its weight to the quartic loss function, $f_3$, since it has the largest curvature for large deviations from optimality. For small deviations, we expect \CAMOO\ to assign weights to the quadratic loss, $f_1$.

    \item \textbf{Selection example instance.} For the selection example instance we expect \CAMOO\ to set the weights as a 1-hot vector on $f_1$, since its the quadratic function with largest curvature across all dimensions. Figure~\ref{fig:app selection camoo} exemplifies this.

\end{itemize}


\begin{figure*}[t]
\vspace{-8pt}
    \centering
    \begin{minipage}{0.45\textwidth}
        \centering
        \includegraphics[width=\textwidth]{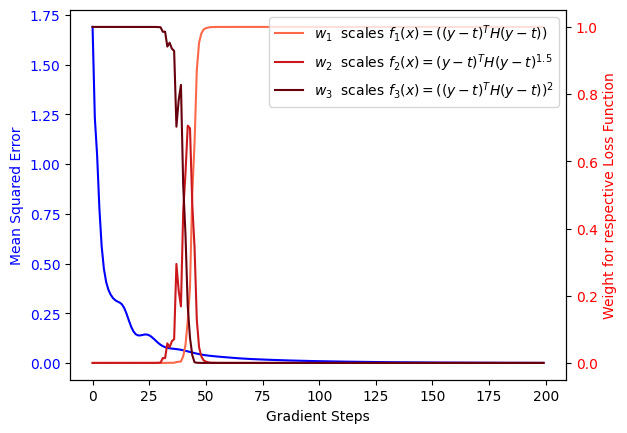}
        \caption{Local curvature example, \CAMOO. The weights flip when the curvature of the loss function changes.} \label{fig:camoo_local}
    \end{minipage}\hfill
    \centering
    \begin{minipage}{0.45\textwidth}
        \centering
        \includegraphics[width=\textwidth]{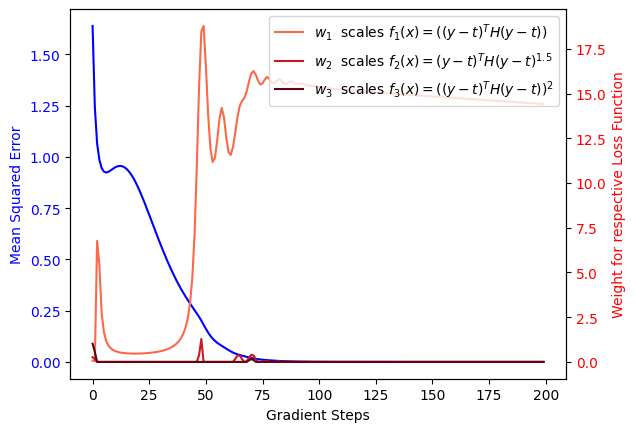} 
        \caption{Local curvature example, \PAMOO.}
    \end{minipage}\hfill

    \vspace{1cm}

        \begin{minipage}{0.45\textwidth}
        \centering
        \includegraphics[width=\textwidth]{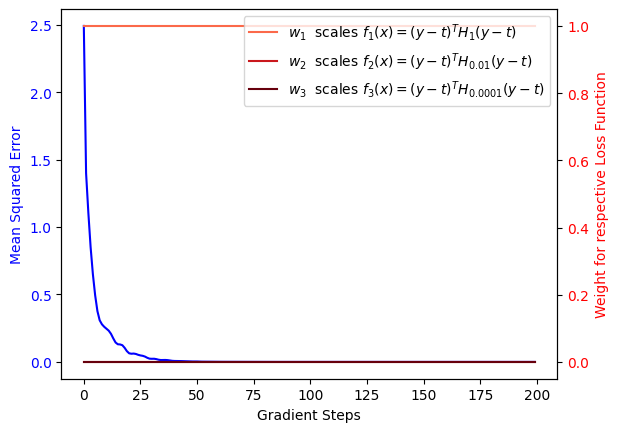}
        \caption{Selection example, \CAMOO. } \label{fig:app selection camoo}
    \end{minipage}\hfill
    \centering
    \begin{minipage}{0.45\textwidth}
        \centering
        \includegraphics[width=\textwidth]{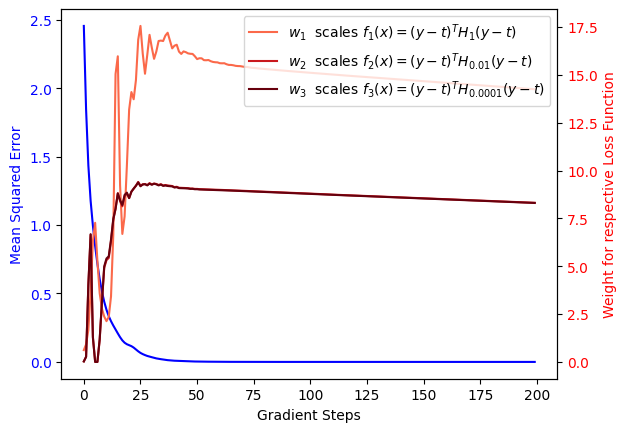} 
        \caption{Selection example, \PAMOO.}
    \end{minipage}\hfill
    
    \label{fig:app_weights_change}
    \caption{Weight vector evolution versus GD iterates.}\label{fig:app_weight_vector_evolution}
\end{figure*}
\newpage
\section{Challenges in Analyzing~\CAMOO}

% \textcolor{red}{YE: decide if we should use Eq.(number) or equation(number). just need to be consistent. } Chose Eq.(number)

\subsection{$f_{\w_k}$ is not a Strongly Convex Function }\label{app:fwk is not strongly convex}

We provide an example that shows that for the AMOO setting, when $\muglobal>0$, the fact that $\lambda_{\min}\brac{\nabla^2 f_{\w_k}(\x_k)}\geq \muglobal$ throughout the iterates of \CAMOO\ does not imply that each $f_{\w_k}$ is $\muglobal$-strongly convex.

The counter example is the local curvature example (see Section~\ref{sec:AMOO setting}), namely,
\begin{align*}
    &f_1(x) = \exp(x)-x, f_2(x) = \exp(-x)+x,
\end{align*}
and $x\in \reals$. The minimum point of both $f_1$ and $f_2$ is at $x=0$. The Hessians of the functions are:
\begin{align}
    &\nabla^2 f_1(x) = \exp(x), \nabla^2 f_2(x) = \exp(-x). \label{eq:app hessian local curvature}
\end{align}
We see that $\nabla^2 f_1(x)>1> \nabla^2 f_2(x)$ for $x>0$, $\nabla^2 f_1(x)<1< \nabla^2 f_2(x)$ for $x<=0$, and $\nabla^2 f_1(0)= \nabla^2 f_2(0)=1$. 

This implies that $\muglobal = 1$, and $\CAMOO$ will set the weight vector as $\w_{+}=(1,0)$ for $x>0$ and $\w_{-}=(0,1)$ for $x\leq0$. However, it is readily observed that neither $f_{\w_{-}}$ or $f_{\w_{+}}$ are $1$-strongly convex functions. The smallest value of the individual Hessians is zero since
\begin{align*}
    &\inf_{x\in \reals}\nabla^2 f_{\w_{-}}(x)= \inf_{x\in \reals}\exp(x)=0\\
    & \inf_{x\in \reals}\nabla^2 f_{\w_{+}}(x)= \inf_{x\in \reals}\exp(-x)=0,
\end{align*}
by Eq.~\eqref{eq:app hessian local curvature}. Hence, the functions $f_{\w_k}$ produced in the iterates of \CAMOO\ are not strongly convex.

\subsection{Weighted function is not necessarily convex}\label{app:naive reduction failure}

We provide a simple counter example that shows failure of a naive reduction in which we construct $f_{\w_\star(\x)}(\x)=\sum_i w_{\star ,i}(\x) f_i(\x)$, where $\w_\star(\x)$ optimizes the curvature at each point via,

$$
\w_\star(\x) \in \argmax_{\w \in \Delta_m} \lambda_{\min} \brac{\sum_{i\in [m]} w_i \nabla^2 f_i(\x_k)} 
$$

and apply gradient descent to the function $f_{\w_\star(\x)}$. The reason such approach is problematic is the fact that $f_{\w_\star(\x)}$ may no longer be a convex function. This is a result of the extra dependence on $\x$ of $\w_\star(\x)$. 

A counter example can be established for a simple scenario in which 
\begin{align*}
    f_1(x) = x^2, f_2(x) = x^2 + c,
\end{align*}
where $x\in \reals,$ for some $c\neq 0$. The two functions are convex, and have a minimizer at $x=0$. However, since the Hessians of the functions are equal, $\nabla^2 f_1(x)= \nabla^2 f_2(x),$ the solution of the optimization problem
\begin{align}
    \label{eq:counter example naive reduction}
    \w_\star(x) \in \argmax_{\w \in \Delta_m} \lambda_{\min} \brac{\sum_{i\in \{1,2\}} w_i \nabla^2 f_i(x)}, 
\end{align}
is arbitrary. Namely, each point on the simplex is a solution of this optimization problem. For example, choosing
\begin{align*}
    \w_\star(x) = (\sin^2(x), \cos^2(x)),
\end{align*}
is a solution of Eq.~\eqref{eq:counter example naive reduction}. With this, the function $f_{\w_\star(x)}$ takes the form of
\begin{align*}
    f_{\w_\star(x)}= x^2 + c \times \cos^2(x),
\end{align*}
which is not a convex function if, for example, $|c|>1$.

Additionally, choosing $\w_\star(x)$ as  non-smooth function, for example
\begin{align*}
    \w_\star(x)=
    \begin{cases}
        (0,1) & x>0\\
        (1,0) & x\leq 0,
    \end{cases}
\end{align*}
results with a non-smooth function $f_{\w_\star(x)}$. This highlights that differentiating the function $f_{\w_\star(x)}$ is flawed from a theoretical perspective:  $f_{\w_\star(x)}$ is not necessarily convex nor smooth.
% Let's define the function $G(\x) = F_{\w}(\x)$, s.t. $\w \in \argmax_{\w \in \Delta_m} \lambda_{min} \brac{\sum_i w_i \nabla^2 f_i(\x_k)} $, and $F_{\w_k}(\x_k)= \sum_i w_i f_i(\x_k)$. It means that for every $\x$ we choose $\w$ that obtains the "argmax" term, which defines the value of $F_{\w_k}(\x_k)$. Therefore $G(\x)$ is a function built from a collection of points, where each point is derived from the previously specified conditions. As a result, There is no reason to think that the $G(\x)$ function is convex. However, $G(\x)$ has a point-wise attribute s.t. for every $\{\w,\x\}$ it holds that 
% \begin{align}
%     \lambda_{\min} \left(\sum_{i=1}^m w_i \nabla^2 f_i(\x) \right)\geq \muglobal. \label{eq:mu_global_definition}
% \end{align}

% Thus, one can wonder if saying something significant about $G(\x)$ is possible. The answer is \emph{No!}. Let's take a simple example in one dimension: $f_1(x) = x^2 +10$, and $f_2(x) = x^2 + x$, both have the same Hessian, i.e. $\nabla^2 f_1(\x) = \nabla^2 f_2(\x)$. Thus, in each point, Algorithm~\ref{alg:AMOOO} can return any $\w$. Therefore, by using Algorithm~\ref{alg:AMOOO-GD} we must more information about $\{f_i\}$.


\section{Preliminaries and Basic Properties}\label{app:pre_and_prp}

In this section, we formally provide our working assumptions. We assume access to multi-objective feedback with $m$ objectives $F(\x) = (f_1(\x),\ldots,f_m(\x))$, when $\forall i \in [m]$ the function $f_i(\x) $ is smooth and self-concordant.  Considering two scenarios AMOO, and  $\epsilon$-AAMOO. In AMOO we assume the functions are aligned in the sense of Eq.~\eqref{eq:aligned_functions}, namely, that they share an optimal solution. In $\epsilon$-AAMOO we assume there is a (non-empty) set of $\epsilon$ approximate solutions in the sense of Eq.~\eqref{eq:Ce_set}, i.e. every solution in the set has a maximum value gap of $\epsilon$ from the minima of every function.

We define the following quantities, for the single and multi objective settings:
\begin{align*}
    &\enorm{\y}^2_{\x} :=\enorm{\y}_{\nabla^2 f(\x)} := \langle \nabla^2 f(\x) \y, \y \rangle \\
    &\enorm{\y}^2_{\x,\w} :=\enorm{\y}_{\nabla^2 f_\w(\x)} := \langle \nabla^2 f_\w(\x) \y, \y \rangle.
\end{align*}
\begin{definition}[Smoothness] \label{ass:smooth}
    $f(\x) : \reals^n \xrightarrow{} \reals$ is called $\beta$-smooth if $~\forall \x, \y \in \reals^n$ the following holds:
    \begin{align}
        f(\y) \leq  f(\x) + \nabla f(\x)^{\top} (\y - \x) + \frac{\beta}{2}  \enorm{ \x - \y } ^2. \nonumber
    \end{align}
\end{definition}

This definition has the following consequence
\begin{lemma}[Standard result, E.g., 9.17~\citet{boyd2004convex}] \label{lemma:smooth-gradient-norm}
    Let $f : \reals^n \to \reals$ a $\beta$-smooth over $\reals^n$, and let $\x_\star \in \argmin_{\x} ~ f(\x)$.  Then, for every $\x \in \reals^n$ it holds that
    \begin{align*}
        \enorm{\nabla f (\x)}^2 \leq 2\beta \brac{f(\x) - f(\x_\star)}.
    \end{align*}
\end{lemma}

% {\color{blue} 
% \begin{definition}[Strong convexity] \label{ass:strong_con}
%     $f(\x) : \reals^n \xrightarrow{} \reals$ is called $\gamma$-strongly convex if $~\forall \x, \y \in \reals^n$ the following holds:
%     \begin{align}
%         f(\y) \geq  f(\x) + \nabla f(\x)^{\top} (\y - \x) + \frac{\gamma}{2}  \enorm{ \x - \y } ^2. \nonumber
%     \end{align}
% \end{definition}

% The following lemma show that for every static weights $\w \in \Delta$, the static function $ \sum_i \w_i f_i(\x)$ is $(\wmin \mu_G)$-strongly convex, where $\wmin = \argmin_i \w$. 
% \begin{lemma}[Standard result, E.g., 9.17~\citet{boyd2004convex}] \label{lemma:smooth-gradient-norm}
%     Let $f : \reals^n \to \reals$ a $\beta$-smooth over $\reals^n$, and let $\x_\star \in \argmin_{\x} ~ f(\x)$.  Then, for every $\x \in \reals^n$ it holds that
%     \begin{align*}
%         \enorm{\nabla f (\x)}^2 \leq 2\beta \brac{f(\x) - f(\x_\star)}.
%     \end{align*}
% \end{lemma}



% }

\begin{definition}[Self-concordant] \label{ass:self_con}
    $f(\x) : \reals^n \xrightarrow{} \reals$ is called self-concordant with parameter $M_{\mathrm{f}} \geq 0$ if $~\forall \x,\y\in \reals^n$ the following holds:
    \begin{align}
        \inner{\nabla^3 f(\x)[\y]\y}{\y}  \preceq 2M_{\mathrm{f}} \enorm{\y}_{\x}^3, \nonumber
    \end{align}
    where $\nabla^3 f(\x)[\y] := \lim_{\alpha\rightarrow 0} \frac{1}{\alpha}\brac{\frac{\nabla^2 f(\x+\alpha \y) - \nabla^2 f(\x)}{\alpha}}$ is the directional derivative of the hessian in~$\y$.
\end{definition}

This definition has the following important consequences.
\begin{lemma}[Theorem 5.1.8 \& Lemma 5.1.5,~\citet{nesterov2013introductory}]\label{lemma:self_con_consequences}
Let $f:\reals^n \rightarrow \reals$ be an $M_{\mathrm{f}}$ self-concordant function. Let $\x, \y \in \reals^n$ , we have
$$
f(\y) \geq f(\x) + \inner{\nabla f(\x)}{\y  - \x} + \frac{1}{M_{\mathrm{f}}^2} \omega\brac{M_{\mathrm{f}}\enorm{\y-\x}_\x },
$$
where $\omega(t) := t-\ln(1-t)$, and, for any $t>0$, $\omega(t)\geq \frac{t^2}{2(1+t)}$.
\end{lemma}
\begin{lemma}[Theorem 5.1.1, ~\citet{nesterov2018lectures}]\label{lemma:sum_of_self_con}
    Let $f_1,f_2 : \reals^n \to \reals$ be $M_{\mathrm{f}}$ self-concordant functions. Let $w_1,w_2 > 0$. Then, $f=w_1 f_1+ w_2 f_2$ is $M = \max_i \{ \frac{1}{\sqrt{w_i}} \} M_{\mathrm{f}}$ self-concordant function.
\end{lemma}
\begin{restatable}[Weighted sum of self-concordant functions]{proposition}{SumSelfCon} \label{prop:sun_of_self_con}
    Let $\{ f_i: \reals^n \to \reals \}_{i=1}^{n} $ be $M_{\mathrm{f}}$ self-concordant functions. Let $\{w_i > 0\}$. Then, $f= \sum_{i=1}^{n} w_i f_i$ is $M = \max_i \{ \frac{1}{\sqrt{w_i}} \} M_{\mathrm{f}}$ self-concordant function.
\end{restatable}
The proof of the last proposition proof is found in Section \ref{app:missing_proofs}.

\begin{theorem}[Weyl's Theorem]\label{thm:weyls} Let $\A$ and $\Delta$ be symmetric matrices in $\reals^{n \times n}$. Let $\lambda_j(\A)$ be the $j^{th}$ largest eigenvalue of a matrix $\A$. Then, for all $j\in [n]$ it holds that $\| \lambda_j(\A) - \lambda_j(\A+\Delta) \| \leq \| \Delta\|_2$, where $\| \Delta\|_2$ is the spectral norm of $\Delta$.
\end{theorem}

\subsection{Auxiliary Results}

Further, we have the following simple consequence of the AMOO setting.
\begin{lemma}\label{lemma:optimality_of_x_star}
For all $\w\in \Delta_m$ and $\x\in \reals^n$ it holds that $f_\w(\x) - f_\w(\x_\star)\geq 0.$
\end{lemma}
\begin{proof}

    Observe that
    $
        f_\w(\x) - f_\w(\x_\star)= \sum_{i=1}^m w_i \brac{f_i(\x) - f_i(\x_\star)}.
    $
    Since $\x_\star$ is the optimal solution for all objectives it holds that $f_i(\x) - f_i(\x_\star) \geq  0.$ The lemma follows from the fact $w_i\geq 0$ for all $i\in [m].$
\end{proof}

\begin{restatable}[Recurrence bound AMOO]{lemma}{ExactIterationBound}
\label{lemma:exact_iteration_bound}
Let $\{ r_k\}_{k\geq 0}$ be a sequence of non-negative real numbers that satisfy the recurrence relation
\begin{align*}
    r_{k+1}^2 \leq r_k^2 -\alpha_1\frac{r_k^2}{1+ \alpha_2 r_k},
\end{align*}
where $\alpha_1\in [0,2)$ and $\alpha_2\in \reals_+.$ Let $k_0 := \Big\lceil \frac{4 \brac{r_0 \alpha_2 - 1}}{ \alpha_1} \Big\rceil$. Then, $r_k$ is bounded by
    \begin{align*}
        r_k \leq 
        \begin{cases}
            r_{k_0} \brac{1-\frac{\alpha_1}{2}}^\frac{k-k_0}{2} & k\geq k_0\\
            r_0 - \frac{ \alpha_1}{4\alpha_2}k & o.w.
        \end{cases}.
    \end{align*}
%     {\color{blue}
% where $\alpha_1\in [0,2)$ and $\alpha_2\in \reals_+.$ Let $k_0 := \Bigg\lceil \frac{\ln{\brac{\frac{1}{r_0^2 \alpha_2^2}}}}{ \ln{\brac{1 - \frac{ \alpha_1}{2\alpha_2 r_0}}}} \Bigg\rceil$. Then, $r_k$ is bounded by
%     \begin{align*}
%         r_k \leq 
%         \begin{cases}
%             r_{k_0} \brac{1-\frac{\alpha_1}{2}}^\frac{k-k_0}{2} & k\geq k_0\\
%             r_0 \brac{1-\frac{\alpha_1}{2\alpha_2 r_0}}^\frac{k}{2} & o.w.
%         \end{cases}.
%     \end{align*}
%     }
\end{restatable}
The proof of the lemma is found in Appendix \ref{app:exact_iteration_bound_proof}\\
The next lemma is for the $\epsilon$-AAMOO setting. We separate them since the recursion and the result of $\epsilon$-AAMOO have more details, making it less readable.


\begin{restatable}[Recurrence bound $\epsilon$-AAMOO]{lemma}{EpsilonIterationBound}\label{lemma:epsilon_app_iteration_bound}
Let $\{ r_k\}_{k\geq 0}$ be a sequence of non-negative real numbers that satisfy the recurrence relation
\begin{align*}
    r_{k+1}^2 \leq r_k^2 -\alpha_1\frac{r_k^2}{1+ \alpha_2 r_k} +\alpha_3 +\alpha_4 r_k,
\end{align*}
where $\alpha_1\in (0,2)$, $\alpha_2\in \reals_+,$ $\alpha_3 \leq \frac{\alpha_1^2}{256\alpha^2_2},$ and $\alpha_4\leq \frac{\alpha_1}{4\alpha_2}$. Let $k_0 := \Big\lceil \frac{16 \brac{r_0 \alpha_2 - 1}}{ \alpha_1} \Big\rceil$. Then, $r_k$ is bounded by
    \begin{align*}
        r_k \leq 
        \begin{cases}
            r_{k_0} \brac{1-\frac{\alpha_1}{2}}^{\frac{k'-k}{2}} + \sqrt{\frac{2\alpha_3}{\alpha_1}+\frac{2\alpha_4}{\alpha_1 \alpha_2}} & k\geq k_0\\
            r_0 - \frac{\alpha_1}{16\alpha_2}k & o.w.
        \end{cases}.
    \end{align*}
\end{restatable}

\section{Proofs of AMOO Results} \label{app:AMOO_results}

See Section~\ref{sec:camoo} for a highlevel description of key steps in the proof. 

We first describe two useful lemmas that are used across the section.

\begin{lemma}[Weighted Function is Self-Concordant]\label{lemma:self_concordant}
For any iteration $k$ of \CAMOO, the function $f_{\w_k}$ is $1/\sqrt{\wmin}M_{\mathrm{f}}$ self-concordant.    
\end{lemma}
\begin{proof}
    This is a direct consequence of Proposition~\ref{prop:sun_of_self_con} and the fact Algorithm~\ref{alg:Weighted-GD} sets the weights by optimizing over a set where the weight vector is lower bounded by $\wmin$.
\end{proof}


\begin{restatable}[Continuity of Minimal Eigenvalue of Hessian]{lemma}{ContOfMinEigenOfHessian}
\label{lemma:wmin_minimal_eigenvalue}
Let $\x\in \mathbb{R}^n$. Further, let $\w_\star \in \argmax\limits_{\w\in \Delta_{m}} \lambda_{\min} \brac{\nabla^2 f_{\w}(\x)}$, $\widehat{\w} \in \argmax\limits_{\w\in \Delta_{m,\wmin}} \lambda_{\min} \brac{\nabla^2 f_{\w}(\x)}$. It holds that $\lambda_{\min}\brac{\nabla^2 f_{\widehat{\w}}(\x)}\geq \lambda_{\min}\brac{\nabla^2 f_{\w_\star}(\x)} - 2m\wmin\beta$.
\end{restatable}

With these two results, we are ready to prove Theorem~\ref{thm:exact_amoo_convergence} and Theorem~\ref{thm:exact_pamoo_convergence}.\\
\subsection{Proof of Theorem~\ref{thm:exact_amoo_convergence}}
Restate it first:
\ExactAmooConvergence*

\begin{proof}
At each iteration Algorithm~\ref{alg:Weighted-GD} gets $\w_k \in\argmax\limits_{\w\in \Delta_{m,w_{\min}}} \lambda_{\min} \brac{\sum_{i} w_i \nabla^2 f_i(\x_{k})}$. Using the assumption that $\max\limits_{\w\in \Delta_m}\lambda_{\min}\brac{\nabla^2 f_{\w_k}(\x_k)} \geq \muglobal$, Lemma~\ref{lemma:wmin_minimal_eigenvalue}, and since we set $w_{\min}=\muglobal/\brac{8m\beta}$ we have that
\begin{align}
    \lambda_{\min} \brac{\nabla^2f_{\w_k}}\geq \lambda_{\min}\brac{\nabla^2f_{\w}} - 2m\wmin\beta \geq \muglobal - \muglobal/4 = (3/4)\muglobal , \label{eq:strongly_convex_param_of_AMOOO}
\end{align}
for all iterations $t$.
Recall that the update rule is given by $\x_{k+1} = \x_k - \eta\nabla f_{\w_k}(\x_k)$, where $\eta$ is the step size.
Then, for every $\x \in \reals^n$ we have
\begin{align}
    \enorm{\x_{k+1}-\x}^2 &= \enorm{\x_k-\eta\nabla f_{\w_k}(\x_k)-\x}^2 \nonumber \\
    &=\enorm{\x_k-\x}^2 - 2\eta\inner{\nabla f_{\w_k}(\x_k)}{\x_k - \x} + \eta^2\enorm{\nabla f_{\w_k}(\x_k)}^2 \label{eq:camoo_gd_recursion}.
\end{align}
By Lemma~\ref{lemma:self_concordant} it holds that $f_{\w_k}$ is 
\begin{align}
    \widehat{M_{\mathrm{f}}} :=1/\sqrt{\wmin} M_{\mathrm{f}}\leq 3\sqrt{m\beta}M_{\mathrm{f}}/\sqrt{\muglobal}\label{eq:self_concordant_param_of_sum}
\end{align}
self-concordant. Then, from Lemma~\ref{lemma:self_con_consequences}, by properties of self-concordant functions, for every $\x \in \reals^n$ we have
\begin{align*}
      \inner{\nabla f_{\w_k}(\x_k)}{\x_k-\x } \geq f_{\w_k}(\x_k) -f_{\w_k}(\x) + \frac{1}{\widehat{M_{\mathrm{f}}}^2} \omega\brac{\widehat{M_{\mathrm{f}}}\enorm{\x - \x_k}_{\x_k,\w_k} },
\end{align*}
Plugging this inequality into Eq.~\eqref{eq:camoo_gd_recursion} implies that
\begin{align}
    \enorm{\x_{k+1}-\x}^2 &\leq \enorm{\x_k-\x}^2 - 2\eta\brac{f_{\w_k}(\x_k) -f_{\w_k}(\x) + \frac{1}{\widehat{M_{\mathrm{f}}}^2} \omega\brac{ \widehat{M_{\mathrm{f}} } \enorm{\x - \x_k}_{\x_k,\w_k} }} + \eta^2\enorm{\nabla f_{\w_k}(\x_k)}^2. \label{eq:camoo_dist_from_x}
\end{align}
Recall that $\x_\star \in \argmin_{\x} f_i(\x)$ for every $i \in [m]$. Since $f_{\w_k}$ is $\beta$-smooth, by using Lemma~\ref{lemma:smooth-gradient-norm}, and plugging in $\x_\star$ we have
\begin{align*}
    &\enorm{\x_{k+1}-\x_\star}^2 \\
    &\leq \enorm{\x_k-\x_\star}^2 - 2\eta\brac{f_{\w_k}(\x_k) -f_{\w_k}(\x_\star) + \frac{1}{\widehat{M_{\mathrm{f}}}^2} \omega\brac{\widehat{M_{\mathrm{f}}}\enorm{\x_\star - \x_k}_{\x_k,\w_k} }} + 2 \beta \eta^2 \brac{f_{\w_k}(\x_k) -f_{\w_k}(\x_\star)} \\
    & =  \enorm{\x_k-\x_\star}^2 - 2\eta \frac{1}{\widehat{M_{\mathrm{f}}}^2} \omega\brac{\widehat{M_{\mathrm{f}}}\enorm{\x_\star - \x_k}_{\x_k,\w_k} } + 2\eta (\beta \eta - 1) \brac{f_{\w_k}(\x_k) -f_{\w_k}(\x_\star)}.
\end{align*}
By using Lemma~\ref{lemma:optimality_of_x_star} it holds that $f_{\w_k}(\x_k) -f_{\w_k}(\x_\star)\geq 0$, and since $0 < \eta \leq 1/2\beta$, it holds that $2\eta (\beta \eta - 1) \brac{f_{\w_k}(\x_k) -f_{\w_k}(\x_\star)} \leq 0$. Then, by using the lower bound from Lemma~\ref{lemma:self_con_consequences}, i.e. $\omega\brac{t} \geq \frac{t^2}{2\brac{1+t}}$, the following holds
\begin{align*}
    \enorm{\x_{k+1}-\x_\star}^2 &\leq \enorm{\x_k-\x_\star}^2 -2\eta \frac{\enorm{\x_\star - \x_k}_{\x_k,\w_k}^2}{1+\widehat{M_{\mathrm{f}}}\enorm{\x_\star - \x_k}_{\x,\w_k}}.
\end{align*}
Note that $\lambda_{\min}\brac{\nabla^2 f_{\w_k}(\x_k)} \enorm{\x_\star - \x_k}^2 \leq \enorm{\x_\star - \x_k}_{\x_k,\w_k}^2 \leq \lambda_{\max}\brac{\nabla^2 f_{\w_k}(\x_k)} \enorm{\x_\star - \x_k}^2$. By using the following: $\lambda_{\min}\brac{\nabla^2 f_{\w_k}(\x_k)} \geq (3/4)\muglobal$ (Eq.~\eqref{eq:strongly_convex_param_of_AMOOO}), $\lambda_{\max}\brac{\nabla^2 f_{\w_k}(\x_k)} \leq \beta$ (smoothness), $\widehat{M_{\mathrm{f}}} \leq 3\sqrt{m\beta}M_{\mathrm{f}} /\sqrt{\muglobal}$ (Eq.~\eqref{eq:self_concordant_param_of_sum}), and $\eta = 1/2\beta$, we obtain
\begin{align*}
    \enorm{\x_{k+1}-\x_\star}^2 &\leq \enorm{\x_k-\x_\star}^2 -\frac{3 \muglobal}{4 \beta} \frac{\enorm{\x_\star - \x_k}^2}{1+\brac{3\sqrt{m}\beta M_{\mathrm{f}}/\sqrt{\muglobal}}\enorm{\x_\star - \x_k}}.
\end{align*}
Now, we are ready for the last step. Denote $\alpha_1 = \frac{3\muglobal}{4\beta}$, and $\alpha_2 = \frac{3\sqrt{m}\beta M_{\mathrm{f}}}{\sqrt{\muglobal}}$. Since $\alpha_1 \in (0,1]$, $\alpha_2 \in \reals_+$, and $\enorm{\x-\x_\star} \in \reals_+$ for every $\x \in \reals^n$, we arrive to the recurrence relation analyzed in Lemma~\ref{lemma:exact_iteration_bound}. Then, we obtain
    \begin{align*}
        \enorm{\x_{k} - \x_\star} \leq 
        \begin{cases}
            \enorm{\x_{k_0} - \x_\star} \brac{1-\frac{3\muglobal}{8\beta}}^{(k-k_0)/2}  & k\geq k_0\\
            \enorm{\x_0 - \x_\star}- k \frac{\muglobal^{3/2}}{16 \beta^2 \sqrt{m} M_{\mathrm{f}}} & o.w.
        \end{cases}
    \end{align*}
where $k_0 := \left\lceil \frac{16 \beta  \brac{\enorm{\x_0 - \x_\star} 3\sqrt{m}\beta M_{\mathrm{f}} -\sqrt{\muglobal}} }{ 3\muglobal^{3/2}}\right\rceil$.
\end{proof}

\subsection{Proof of Theorem~\ref{thm:exact_pamoo_convergence}}
Restate it first:
\ExactPAmooConvergence*

\begin{proof}
Recall that for every $\w\in \reals^m_+$ it holds that $f_{\w}$ is a convex function. Hence, for every $\x,\y \in \reals^n$ it holds that
\begin{align*}
    &f_{\w}(\x) - f_{\w}(\y)  \leq \nabla f_\w(\x)^T(\x-\y). 
\end{align*}
Recall that the step size $\eta = 1$, then the update rule is given by $\x_{k+1} = \x_k - \nabla f_{\w_k}(\x_k)$. Then, by using the previous equation, for every $\x \in \reals^n$ we have
\begin{align}
    \enorm{\x_{k+1}-\x}^2 &=\enorm{\x_k-\x}^2 - 2\inner{\nabla f_{\w_k}(\x_k)}{\x_k - \x} + \enorm{\nabla f_{\w_k}(\x_k)}^2 \nonumber\\
    &\leq \enorm{\x_k-\x}^2 - 2 \brac{f_{\w_k}(\x_k)- f_{\w_k} (\x)} +\enorm{\nabla f_{\w_k}(\x_k)}^2 , \label{eq:PAMOO_dist_from_x}
\end{align}
Recall that $\x_\star \in \argmin_{\x \in \reals^n} f_i(\x)$ for every $i \in [m]$. Since the update rule of \texttt{PAMOO} is 
$$
\w_k\in \argmax_{\w\in \reals^m_+} 2\brac{f_{\w_k}(\x_k)- f_{\w_k} (\x_\star)} - \enorm{\nabla f_{\w_k}(\x_k)}^2,
$$
the following holds
\begin{align}
    \enorm{\x_{k+1}-\x_\star}^2 &\leq \enorm{\x_k-\x_\star}^2 -  \max_{\w \in \reals_+^m} \Big{\{} 2\brac{f_{\w}(\x_k)- f_{\w} (\x_\star)} - \enorm{\nabla f_{\w}(\x_k)}^2 \Big{\}}, \label{eq:PAMOO_dist_from_opt}
\end{align}
Denote $\w_\star = \argmax\limits_{\w\in \Delta_{m,\wmin}} \lambda_{\min}\brac{\sum_{i=1}^m w_i \nabla^2 f_i(\x_\star)}$, $a_k = f_{\w_\star}(\x_k)- f_{\w_\star} (\x_\star)$, and $b_k = \enorm{\nabla f_{\w_\star}(\x_k)}^2$. Let $w(\x_k) = \w_\star \frac{a_k}{b_k} \in \reals^m_+$, we can lower bound of the last expression as follows
\begin{align*}
    \max_{\w\in \reals_+^m} \left[ 2\brac{f_{\w}(\x_k)- f_{\w} (\x_\star)} - \enorm{\nabla f_{\w}(\x_k)}^2 \right] & \geq 2\brac{f_{\w(\x_k)}(\x_k)- f_{\w(\x_k)} (\x_\star)}  -\enorm{\nabla f_{\w(\x_k)}(\x_k)}^2 \\
    & =   \frac{\brac{f_{\w_\star}(\x_k)- f_{\w_\star} (\x_\star)}^2}{\enorm{\nabla f_{\w_\star}(\x_k)}^2}.
\end{align*}
Since $\w_\star\in \Delta_{m,\wmin}$ it holds that $f_{\w_\star}$ is $\beta$ smooth. Then, it holds that $\enorm{\nabla f_{\w_\star}(\x)}^2 \leq 2\beta \brac{f_{\w_\star}(\x)- f_{\w_\star} (\x_\star)}$ for every $\x$, and we have
\begin{align*}
     \max_{\w\in \reals_+^m} \left[ 2\brac{f_{\w}(\x_k)- f_{\w} (\x_\star)} - \enorm{\nabla f_{\w}(\x_k)}^2 \right] & \geq \frac{f_{\w_\star}(\x_k)- f_{\w_\star} (\x_\star)}{2 \beta} 
\end{align*}
Plugging this in Eq.~\eqref{eq:PAMOO_dist_from_opt}, we arrive to 
\begin{align*}
    \enorm{\x_{k+1}-\x_\star}^2 &\leq \enorm{\x_k-\x_\star}^2 -  \frac{ f_{\w_\star}(\x_k)- f_{\w_\star} (\x_\star)}{2 \beta}
\end{align*}
By Lemma~\ref{lemma:self_concordant} it holds that $f_{\w_\star}$ is $\widehat{M_{\mathrm{f}}}:=1/\sqrt{\wmin} M_{\mathrm{f}}$ self concordant. Then, From Lemma~\ref{lemma:self_con_consequences}, and its lower bound , i.e. $\omega\brac{t} \geq \frac{t^2}{2\brac{1+t}}$, we have
\begin{align*}
       f_{\w_\star}(\x_k) -f_{\w_\star}(\x_\star) \geq \inner{\nabla f_{\w_\star}(\x_\star)}{\x_k - \x_\star} +  \frac{\enorm{\x_k - \x_\star}_{ \x_\star,\w_\star}^2}{2\brac{1+\widehat{M_{\mathrm{f}}}\enorm{\x_k - \x_\star}_{\x_\star,\w_\star}}} = \frac{\enorm{\x_k - \x_\star}_{ \x_\star,\w_\star}^2}{2\brac{1+\widehat{M_{\mathrm{f}}}\enorm{\x_k - \x_\star}_{\x_\star,\w_\star}}}.
\end{align*}
The equality is due to the optimality condition, $\nabla f_i(\x_\star)=0$ for every $i \in [m]$, thus, $\nabla f_{\w_\star}(\x_\star) = \bold{0}$.
Combining the last two equations, we have 
\begin{align*}
    \enorm{\x_{k+1}-\x_\star}^2 &\leq \enorm{\x_k-\x_\star}^2 -  \frac{1}{4 \beta} \frac{\enorm{\x_k - \x_\star}_{ \x_\star,\w_\star}^2}{1+\widehat{M_{\mathrm{f}}}\enorm{\x_k - \x_\star}_{\x_\star,\w_\star}}
\end{align*}
Note that $\lambda_{\min}\brac{\nabla^2 f_{\w_\star}(\x_\star)} \enorm{\x_\star - \x_k}^2 \leq \enorm{\x_\star - \x_k}_{\x_\star,\w_\star}^2 \leq \lambda_{\max}\brac{\nabla^2 f_{\w_\star}(\x_\star)} \enorm{\x_\star - \x_k}^2$. Since $\lambda_{\max}\brac{\nabla^2 f_{\w_\star}(\x_\star)} \leq \beta$ (smoothness), and since $w_{\min}= \mulocal /(8m\beta)$, then $\widehat{M_{\mathrm{f}}} \leq 3\sqrt{m\beta}M_{\mathrm{f}} /\sqrt{\mulocal}$. Thus, it holds that
\begin{align*}
    \enorm{\x_{k+1}-\x_\star}^2 &\leq \enorm{\x_k-\x_\star}^2 -  \frac{1}{4 \beta} \frac{\lambda_{\min}\brac{\nabla^2 f_{\w_\star}(\x_\star)} \enorm{\x_\star - \x_k}^2}{1+ \frac{3\sqrt{m} M_{\mathrm{f}} \beta}{\sqrt{\mulocal}}  \enorm{\x_k - \x_\star}}
\end{align*}
Using the assumption that $\max\limits_{\w\in \Delta_m}\lambda_{\min}\brac{\nabla^2 f_{\w}(\x_\star)} \geq \mulocal$, Lemma~\ref{lemma:wmin_minimal_eigenvalue}, we have that
\begin{align*}
    \lambda_{\min} \brac{\nabla^2f_{\w_\star}(\x_\star)}\geq \max\limits_{\w\in \Delta_m}\lambda_{\min}\brac{\nabla^2 f_{\w}(\x_\star)} - 2m\wmin\beta \geq \mulocal - \mulocal/4 = (3/4)\mulocal.
\end{align*}
Finally, we obtain the recurring equation we wish:
\begin{align*}
    \enorm{\x_{k+1}-\x_\star}^2 &\leq \enorm{\x_k-\x_\star}^2 -  \frac{3 \mulocal}{16 \beta} \frac{ \enorm{\x_\star - \x_k}^2}{1+ \frac{3\sqrt{m} M_{\mathrm{f}} \beta}{\sqrt{\mulocal}}  \enorm{\x_k - \x_\star}}
\end{align*} 
Denote $\alpha_1 = \frac{3\mulocal}{16\beta}$, and $\alpha_2 = \frac{3\sqrt{m}\beta M_{\mathrm{f}}}{\sqrt{\mulocal}}$. Note that $\alpha_1 \in (0,1]$, $\alpha_2 \in \reals_+$, and $\enorm{\x-\x_\star} \in \reals_+$ for every $\x \in \reals^n$, we arrive to the recurrence relation analyzed in Lemma~\ref{lemma:exact_iteration_bound}. Then, we obtain
\begin{align*}
    \enorm{\x_{k} - \x_\star} \leq 
    \begin{cases}
        \enorm{\x_{k_0} - \x_\star} \brac{1-\frac{3\mulocal}{32\beta}}^{(k-k_0)/2}  & k\geq k_0\\
        \enorm{\x_0 - \x_\star}- k \frac{\mulocal^{3/2}}{64 \beta^2 \sqrt{m} M_{\mathrm{f}}} & o.w.
    \end{cases}
\end{align*}
where $k_0 := \left\lceil \frac{64 \beta  \brac{\enorm{\x_0 - \x_\star} 3\sqrt{m}\beta M_{\mathrm{f}} -\sqrt{\mulocal}} }{ 3\mulocal^{3/2}}\right\rceil$.
\end{proof}

\section{$\epsilon$-Approximation Solution}\label{app:epsilon_app_sol}

% \begin{definition}[$\epsilon$-Approximate Solution Set] \label{def:epsilon_app_solution_set}
%      Let $\epsilon \geq 0$. $\mC_\epsilon$ is $\epsilon$-Approximate Solution Set ($\epsilon$-ASS) if for every $i \in [m]$ it holds that $f_i(\x) - f_i(\x_{\star}^i) \leq \epsilon$, i.e.
%     \begin{align*}
%         \mC_\epsilon = \{ \x \in \reals^n | \ f_i(\x) - f_i(\x_{\star}^i) \leq \epsilon ~~ \forall i\in[m] \},
%     \end{align*}
%     where $\x_\star^i \in \argmin_{\x \in \reals^n} \{ f_i(\x) \}$.
% \end{definition}

In this section, we represent the formal theorems of the Informal Theorem~\ref{thm:informal_epsilon_AAMOO} for \CAMOO ~and \PAMOO. First, we
rewrite the definition of $\epsilon$- approximate solutions set.

\begin{definition}[$\epsilon$-Approximate Solution Set] \label{def:epsilon_app_solution_set}
     Let $\epsilon \geq 0$. $\mC_\epsilon$ is $\epsilon$-Approximate Solution Set ($\epsilon$-ASS) if for every $i \in [m]$ it holds that $f_i(\x) - f_i(\x_{\star}^i) \leq \epsilon$, i.e.
    \begin{align*}
        \mC_\epsilon = \{ \x \in \reals^n | \ f_i(\x) - f_i(\x_{\star}^i) \leq \epsilon ~~ \forall i\in[m] \},
    \end{align*}
    where $\x_\star^i \in \argmin_{\x \in \reals^n} \{ f_i(\x) \}$.
\end{definition}

We show in the following formal theorem that for $\epsilon>0$ \CAMOO ~converges for any chosen point from the set $\mC_\epsilon$, i.e. the $\epsilon$- approximate solutions set.

\begin{restatable}[$\muglobal$ Approximation Convergence of \CAMOO]{theorem}{EpsilonCAmooConvergence}
\label{thm:epsilon_camoo_convergence}
        Suppose $\{f_i\}_{i\in [m]}$ are $\beta$ smooth, $M_{\mathrm{f}}$ self-concordant, $\mC_\epsilon$ is an $\epsilon$-ASS and that $\muglobal > 0$. Let $k_0 := \left\lceil \frac{64 \beta  \brac{\frac{3 \sqrt{m}\beta M_{\mathrm{f}} \enorm{\x_0 - \xse} }{\sqrt{\muglobal}}-1} }{ 3\muglobal}\right\rceil$, where $\enorm{\cdot}$ is the 2-norm. Let $ \frac{\muglobal^3 }{4^6 m \beta^3 M_{\mathrm{f}}^2} \geq \epsilon > 0$. Then, for every point $\xse \in \mC_\epsilon$, \texttt{Weighted-GD} instantiated with \CAMOO\ weight-optimizer and $\eta = 1/2\beta$ converges with rate:
    \begin{align*}
        \enorm{\x_{k} - \xse} \leq 
        \begin{cases}
            \enorm{\x_{k_0} - \xse} \brac{1-\frac{3\muglobal}{8\beta}}^{(k-k_0)/2} + \sqrt{\frac{8  }{ 3 \muglobal}\epsilon} & k\geq k_0\\
            \enorm{\x_0 - \xse}- k \frac{\muglobal^{3/2}}{4^3 \beta^2 \sqrt{m} M_{\mathrm{f}}} & o.w.
        \end{cases}
    \end{align*}
\end{restatable}

\begin{proof}
Let $\xse \in \mC_\epsilon$. Denote $\x_k^\star = \argmin_{\x\in\reals^n} f_{\w_k}(\x)$ for every $k$, then since $f_{\w_k}$ is $\beta$-smooth, by using Lemma~\ref{lemma:smooth-gradient-norm}, it holds that $\enorm{\nabla f (\x)}^2 \leq 2\beta \brac{f(\x) - f(\x_\star)}$. Plugging in $\x = \xse$ in Eq.~\eqref{eq:camoo_dist_from_x}, we have 
\begin{align*}
    &\enorm{\x_{k+1}-\xse}^2 \\
    &\leq \enorm{\x_k-\xse}^2 - 2\eta\brac{f_{\w_k}(\x_k) -f_{\w_k}(\xse) + \frac{1}{\widehat{M_{\mathrm{f}}}^2} \omega\brac{\widehat{M_{\mathrm{f}}}\enorm{\xse - \x_k}_{\x_k,\w_k} }} + 2 \beta \eta^2 \brac{f_{\w_k}(\x_k) -f_{\w_k}(\x_k^\star)} \\
    & =  \enorm{\x_k-\xse}^2 - 2\eta \frac{1}{\widehat{M_{\mathrm{f}}}^2} \omega\brac{\widehat{M_{\mathrm{f}}}\enorm{\xse - \x_k}_{\x_k,\w_k} } \\
    &\quad + 2\eta \brac{f_{\w_k}(\xse) -f_{\w_k}(\x_k^\star)} + 2\eta (\beta \eta - 1) \brac{f_{\w_k}(\x_k) -f_{\w_k}(\x_k^\star)}.
\end{align*}
Since $f_{\w_k}(\x_k) -f_{\w_k}(\x_k^\star)\geq 0$, and since $0 < \eta \leq 1/2\beta$, it holds that $2\eta (\beta \eta - 1) \brac{f_{\w_k}(\x_k) -f_{\w_k}(\x_k^\star)} \leq 0$. In addition, by using the lower bound from Lemma~\ref{lemma:self_con_consequences}, i.e. $\omega\brac{t} \geq \frac{t^2}{2\brac{1+t}}$, and Definition~\ref{def:epsilon_app_solution_set} with the fact that $\sum_i w_i = 1$, the following holds
\begin{align*}
    \enorm{\x_{k+1}-\xse}^2 &\leq \enorm{\x_k-\xse}^2 -2\eta \frac{\enorm{\xse - \x_k}_{\x_k,\w_k}^2}{1+\widehat{M_{\mathrm{f}}}\enorm{\xse - \x_k}_{\x,\w_k}} + 2\eta\epsilon.
\end{align*}
Note that $\lambda_{\min}\brac{\nabla^2 f_{\w_k}(\x_k)} \enorm{\xse - \x_k}^2 \leq \enorm{\xse - \x_k}_{\x_k,\w_k}^2 \leq \lambda_{\max}\brac{\nabla^2 f_{\w_k}(\x_k)} \enorm{\xse - \x_k}^2$. By using the following: $\lambda_{\min}\brac{\nabla^2 f_{\w_k}(\x_k)} \geq (3/4)\muglobal$ (Eq.~\eqref{eq:strongly_convex_param_of_AMOOO}, $\lambda_{\max}\brac{\nabla^2 f_{\w_k}(\x_k)} \leq \beta$ (smoothness), $\widehat{M_{\mathrm{f}}} \leq 3\sqrt{m\beta}M_{\mathrm{f}} /\sqrt{\muglobal}$ (Eq.~\eqref{eq:self_concordant_param_of_sum}), and $\eta = 1/2\beta$, we obtain
\begin{align*}
    \enorm{\x_{k+1}-\xse}^2 &\leq \enorm{\x_k-\xse}^2 -\frac{3 \muglobal}{4 \beta} \frac{\enorm{\xse - \x_k}^2}{1+\brac{3\sqrt{m}\beta M_{\mathrm{f}}/\sqrt{\muglobal}}\enorm{\xse - \x_k}} + \frac{\epsilon}{\beta}.
\end{align*}
Now, we are ready for the last step. Denote $\alpha_1 = \frac{3\muglobal}{4\beta}$, $\alpha_2 = \frac{3\sqrt{m}\beta M_{\mathrm{f}}}{\sqrt{\muglobal}}$, and $\alpha_3 = \frac{\epsilon}{\beta}$. Since $\alpha_1 \in (0,2)$, $\alpha_2 \in \reals_+$, $\alpha_3 \leq \frac{\alpha_1^2}{256\alpha^2_2}$ and $\enorm{\x-\xse} \in \reals_+$ for every $\x \in \reals^n$, we arrive to the recurrence relation analyzed in Lemma~\ref{lemma:epsilon_app_iteration_bound}. Then, we obtain
    \begin{align*}
        \enorm{\x_{k} - \xse} \leq 
        \begin{cases}
            \enorm{\x_{k_0} - \xse} \brac{1-\frac{3\muglobal}{8\beta}}^{(k-k_0)/2} + \sqrt{\frac{8  }{ 3 \muglobal}\epsilon} & k\geq k_0\\
            \enorm{\x_0 - \xse}- k \frac{\muglobal^{3/2}}{4^3 \beta^2 \sqrt{m} M_{\mathrm{f}}} & o.w.
        \end{cases}
    \end{align*}
where $k_0 := \left\lceil \frac{64 \beta  \brac{\frac{3 \sqrt{m}\beta M_{\mathrm{f}} \enorm{\x_0 - \xse} }{\sqrt{\muglobal}}-1} }{ 3\muglobal}\right\rceil$.
\end{proof}

Before we continue to \PAMOO, we recall Definition~\ref{def:mulocaleps} which defines $\mulocaleps$. This parameter is the maximum curvature over the $\epsilon$-approximate solutions set, which can be much greater than $\muglobal$, and $\mulocal$. Before we show the formal theorem of \PAMOO, we define $\widehat{\xse} \in \mC_\epsilon$ which is the point with the maximum curvature, s.t.
\begin{align*}
    \widehat{\xse} = \argmax_{\xse \in \mC_\epsilon} \max_{\w \in \Delta_m} \lambda_{\min}\left(\sum_{i=1}^m w_i \nabla^2 f_i(\xse) \right), ~~~~~ \mulocaleps =  \max_{\w \in \Delta_m} \lambda_{\min}\left(\sum_{i=1}^m w_i \nabla^2 f_i(\widehat{\xse}) \right).
\end{align*}
Now, we show the formal theorem that for $\epsilon>0$ \PAMOO ~converges to $\widehat{\xse}$.
\begin{restatable}[$\mulocaleps$ Approximation Convergence of \PAMOO]{theorem}{EpsilonPAmooConvergence}
\label{thm:epsilon_pamoo_convergence}
    Suppose $\{f_i\}_{i\in [m]}$ are $\beta$ smooth, $M_{\mathrm{f}}$ self-concordant, $\mC_\epsilon$ is an $\epsilon$-ASS and that $\mulocaleps > 0$, where $\min \big\{ \frac{\beta}{8} , \frac{1}{2 \beta} \big\} \frac{\mulocaleps^3}{4^4 \beta^4 m M_{\mathrm{f}}^2}\geq \epsilon > 0$. Let $k_0 := \left\lceil \frac{4^4  \beta  \brac{\enorm{\x_0 - \widehat{\xse}} \frac{3\sqrt{m}\beta M_{\mathrm{f}}}{\sqrt{\mulocaleps }} -1} }{ 3\mulocaleps}\right\rceil$ where $\enorm{\cdot}$ is the Euclidean-norm. Then, \texttt{Weighted-GD} instantiated with \PAMOO\ weight-optimizer and $\eta = 1$  converges to $\widehat{\xse}$ with rate:
    \begin{align*}
        \enorm{\x_{k} - \widehat{\xse}} \leq 
        \begin{cases}
            \enorm{\x_{k_0} - \widehat{\xse}} \brac{1-\frac{3\mulocaleps}{32\beta}}^\frac{k-k_0}{2} + \sqrt{\frac{16\epsilon}{3\mulocaleps}+\frac{32 \sqrt{2\beta \epsilon}}{9 \sqrt{\mulocal m} M_{\mathrm{f}}}}  & k\geq k_0\\
            \enorm{\x_0 - \widehat{\xse}}- k \frac{\mulocal^{3/2}}{64 \beta^2 \sqrt{m} M_{\mathrm{f}}} & o.w.
        \end{cases}
    \end{align*}
\end{restatable}

\begin{proof}
Combining Eq.~\eqref{eq:PAMOO_dist_from_x} with the update rule of \texttt{PAMOO}, and plugging in $\widehat{\xse}$, i.e. 
$$
\w_k\in \argmax_{\w\in \reals^m_+} 2\brac{f_{\w_k}(\x_k)- f_{\w_k} (\widehat{\xse})} - \enorm{\nabla f_{\w_k}(\x_k)}^2,
$$
the following holds
\begin{align}
    \enorm{\x_{k+1}-\widehat{\xse}}^2 &\leq \enorm{\x_k-\widehat{\xse}}^2 -  \max_{\w \in \reals_+^m} \Big{\{} 2\brac{f_{\w}(\x_k)- f_{\w} (\widehat{\xse})} - \enorm{\nabla f_{\w}(\x_k)}^2 \Big{\}} \label{eq:epsilon_PAMOO_dist_from_opt}
\end{align}
Denote $\wse = \argmax\limits_{\w\in \Delta_{m,\wmin}} \lambda_{\min}\brac{\sum_{i=1}^m w_i \nabla^2 f_i(\widehat{\xse})}$, $a_k = f_{\wse}(\x_k)- f_{\wse} (\widehat{\xse})$, and $b_k = \enorm{\nabla f_{\wse}(\x_k)}^2$. Let $w(\x_k) = \wse \frac{a_k}{b_k} \in \reals^m_+$, we can lower bound of the last expression as follows
\begin{align*}
    \max_{\w\in \reals_+^m} \left[ 2\brac{f_{\w}(\x_k)- f_{\w} (\widehat{\xse})} - \enorm{\nabla f_{\w}(\x_k)}^2 \right] & \geq 2\brac{f_{\w(\x_k)}(\x_k)- f_{\w(\x_k)} (\widehat{\xse})}  -\enorm{\nabla f_{\w(\x_k)}(\x_k)}^2 \\
    & =   \frac{\brac{f_{\wse}(\x_k)- f_{\wse} (\widehat{\xse})}^2}{\enorm{\nabla f_{\wse}(\x_k)}^2}.
\end{align*}
Denote $\x_\star \in \argmin_\x f_{\wse}(\x) $. Then, it holds that 
\begin{align*}
    &\frac{\brac{f_{\wse}(\x_k)- f_{\wse} (\widehat{\xse})}^2}{\enorm{\nabla f_{\wse}(\x_k)}^2} \\
    & =   \frac{\brac{f_{\wse}(\x_k)- f_{\wse} (\x_\star) + f_{\wse}(\x_\star)- f_{\wse} (\widehat{\xse})}\brac{f_{\wse}(\x_k)- f_{\wse} (\widehat{\xse})}}{\enorm{\nabla f_{\wse}(\x_k)}^2}\\
    & =   \frac{\brac{f_{\wse}(\x_k)- f_{\wse} (\x_\star)}\brac{f_{\wse}(\x_k)- f_{\wse} (\widehat{\xse})}}{\enorm{\nabla f_{\wse}(\x_k)}^2} + \frac{\brac{ f_{\wse}(\x_\star)- f_{\wse} (\widehat{\xse})}\brac{f_{\wse}(\x_k)- f_{\wse} (\widehat{\xse})}}{\enorm{\nabla f_{\wse}(\x_k)}^2}\\
    & =   \frac{\brac{f_{\wse}(\x_k)- f_{\wse} (\x_\star)}\brac{f_{\wse}(\x_k)- f_{\wse} (\widehat{\xse})}}{\enorm{\nabla f_{\wse}(\x_k)}^2} + \frac{\brac{ f_{\wse}(\x_\star)- f_{\wse} (\widehat{\xse})}\brac{f_{\wse}(\x_k)- f_{\wse} (\x_\star)}}{\enorm{\nabla f_{\wse}(\x_k)}^2} \\
    & ~~~~ + \frac{\brac{ f_{\wse}(\x_\star)- f_{\wse} (\widehat{\xse})}^2}{\enorm{\nabla f_{\wse}(\x_k)}^2}\\
    & \geq \frac{\brac{f_{\wse}(\x_k)- f_{\wse} (\x_\star)}\brac{f_{\wse}(\x_k)- f_{\wse} (\widehat{\xse})}}{\enorm{\nabla f_{\wse}(\x_k)}^2} + \frac{\brac{ f_{\wse}(\x_\star)- f_{\wse} (\widehat{\xse})}\brac{f_{\wse}(\x_k)- f_{\wse} (\x_\star)}}{\enorm{\nabla f_{\wse}(\x_k)}^2}.
\end{align*}
Since $\wse\in \Delta_{m,\wmin}$ it holds that $f_{\wse}$ is $\beta$ smooth. Then, it holds that $\enorm{\nabla f_{\wse}(\x)}^2 \leq 2\beta \brac{f_{\wse}(\x)- f_{\wse} (\x_\star)}$ for every $\x$, and we have
\begin{align*}
     \max_{\w\in \reals_+^m} \left[ 2\brac{f_{\w}(\x_k)- f_{\w} (\widehat{\xse})} - \enorm{\nabla f_{\w}(\x_k)}^2 \right] & \geq \frac{f_{\wse}(\x_k)- f_{\wse} (\widehat{\xse})}{2 \beta} + \frac{ f_{\wse}(\x_\star)- f_{\wse} (\widehat{\xse})}{2\beta}.
\end{align*}
Plugging this in Eq.~\eqref{eq:epsilon_PAMOO_dist_from_opt}, we arrive to 
\begin{align*}
    \enorm{\x_{k+1}-\widehat{\xse}}^2 &\leq \enorm{\x_k-\widehat{\xse}}^2 -  \frac{ f_{\wse}(\x_k)- f_{\wse} (\widehat{\xse})}{2 \beta} + \frac{ f_{\wse} (\widehat{\xse}) - f_{\wse}(\x_\star)}{2\beta}\\
    &\leq \enorm{\x_k-\widehat{\xse}}^2 -  \frac{ f_{\wse}(\x_k)- f_{\wse} (\widehat{\xse})}{2 \beta} + \frac{ \epsilon}{2\beta}.
\end{align*}
By Lemma~\ref{lemma:self_concordant} it holds that $f_{\w_\star}$ is $\widehat{M_{\mathrm{f}}}:=1/\sqrt{\wmin} M_{\mathrm{f}}$ self concordant. Then, From Lemma~\ref{lemma:self_con_consequences}, and its lower bound , i.e. $\omega\brac{t} \geq \frac{t^2}{2\brac{1+t}}$, we have
\begin{align*}
       f_{\wse}(\x_k) -f_{\wse}(\widehat{\xse}) & \geq \inner{\nabla f_{\wse}(\widehat{\xse})}{\x_k - \widehat{\xse}} +  \frac{\enorm{\x_k - \widehat{\xse}}_{ \widehat{\xse},\wse}^2}{2\brac{1+\widehat{M_{\mathrm{f}}}\enorm{\x_k - \widehat{\xse}}_{\widehat{\xse},\wse}}} \\
       & \geq -\enorm{\nabla f_{\wse}(\widehat{\xse})} \enorm{\x_k - \widehat{\xse}} +  \frac{\enorm{\x_k - \widehat{\xse}}_{ \widehat{\xse},\wse}^2}{2\brac{1+\widehat{M_{\mathrm{f}}}\enorm{\x_k - \widehat{\xse}}_{\widehat{\xse},\wse}}} .
\end{align*}
By Lemma~\ref{lemma:smooth-gradient-norm}, we have that $\enorm{\nabla f_{\wse}(\widehat{\xse})}^2 \leq 2\beta \brac{f_{\wse}(\widehat{\xse})- f_{\wse} (\x_\star)}\leq 2\beta \epsilon$, and, hence, $-\enorm{\nabla f_{\wse}(\widehat{\xse})}\geq -\sqrt{2\beta\epsilon}$. Plugging this back results with the following
\begin{align*}
    \enorm{\x_{k+1}-\widehat{\xse}}^2 & \leq \enorm{\x_k-\widehat{\xse}}^2 -  \frac{\enorm{\x_k - \widehat{\xse}}_{ \widehat{\xse},\wse}^2}{4\beta \brac{1+\widehat{M_{\mathrm{f}}} \enorm{\x_k-\widehat{\xse}}_{\widehat{\xse}, \wse}}} + \frac{ \epsilon}{2\beta} + \sqrt{2 \beta \epsilon} \enorm{\x_k - \widehat{\xse}}
\end{align*}
Note that $\lambda_{\min} \brac{\nabla^2 f_{\wse}(\widehat{\xse})} \enorm{\widehat{\xse} - \x_k}^2 \leq \enorm{\widehat{\xse} - \x_k}_{\widehat{\xse},\wse}^2 \leq \lambda_{\max} \brac{\nabla^2 f_{\wse}(\widehat{\xse})} \enorm{\widehat{\xse} - \x_k}^2$. Since $\lambda_{\max} \brac{\nabla^2 f_{\wse}(\widehat{\xse})} \leq \beta$ (smoothness), and since $w_{\min}= \mulocaleps /(8m\beta)$, then $\widehat{M_{\mathrm{f}}} \leq 3\sqrt{m\beta}M_{\mathrm{f}} /\sqrt{\mulocaleps}$. Thus, it holds that
\begin{align*}
    \enorm{\x_{k+1}-\widehat{\xse}}^2 &\leq \enorm{\x_k-\widehat{\xse}}^2 -  \frac{1}{4 \beta} \frac{\lambda_{\min}\brac{\nabla^2 f_{\wse}(\widehat{\xse})} \enorm{\widehat{\xse} - \x_k}^2}{1+ \frac{3\sqrt{m} M_{\mathrm{f}} \beta}{\sqrt{\mulocaleps}}  \enorm{\x_k - \widehat{\xse}}} + \frac{ \epsilon}{2\beta} + \sqrt{2 \beta \epsilon} \enorm{\x_k - \widehat{\xse}}
\end{align*}
Using the assumption that $\max\limits_{\w\in \Delta_m}\lambda_{\min}\brac{\nabla^2 f_{\w}(\widehat{\xse})} = \mulocaleps$, Lemma~\ref{lemma:wmin_minimal_eigenvalue}, we have that
\begin{align*}
    \lambda_{\min} \brac{\nabla^2f_{\wse}(\widehat{\xse})}\geq \max\limits_{\w\in \Delta_m}\lambda_{\min}\brac{\nabla^2 f_{\w}(\widehat{\xse})} - 2m\wmin\beta \geq \mulocaleps - \mulocaleps/4 = (3/4)\mulocaleps.
\end{align*}
Finally, we obtain the recurring equation we wish:
\begin{align*}
    \enorm{\x_{k+1}-\widehat{\xse}}^2 &\leq \enorm{\x_k-\widehat{\xse}}^2 -  \frac{3\mulocaleps}{16 \beta} \frac{ \enorm{\widehat{\xse} - \x_k}^2}{1+ \frac{3\sqrt{m} M_{\mathrm{f}} \beta}{\sqrt{\mulocaleps}}  \enorm{\x_k - \widehat{\xse}}} + \frac{ \epsilon}{2\beta} + \sqrt{2 \beta \epsilon} \enorm{\x_k - \widehat{\xse}}
\end{align*}
Denote $\alpha_1 = \frac{3\mulocaleps}{16\beta}$, $\alpha_2 = \frac{3\sqrt{m}\beta M_{\mathrm{f}}}{\sqrt{\mulocaleps }}$, $\alpha_3 = \frac{ \epsilon}{2\beta} $, and $\alpha_4 = \sqrt{2 \beta \epsilon}$. Note that $\alpha_1 \in (0,1)$, $\alpha_2 \in \reals_+$, $\alpha_3 \leq \frac{\alpha_1^2}{256\alpha^2_2},$ and $\alpha_4\leq \frac{\alpha_1}{4\alpha_2}.$ and $\enorm{\x-\widehat{\xse}} \in \reals_+$ for every $\x \in \reals^n$, we arrive to the recurrence relation analyzed in Lemma~\ref{lemma:epsilon_app_iteration_bound}. Then, we obtain
\begin{align*}
    \enorm{\x_{k} - \widehat{\xse}} \leq 
    \begin{cases}
        \enorm{\x_{k_0} - \widehat{\xse}} \brac{1-\frac{3\mulocaleps}{32\beta}}^\frac{k-k_0}{2} + \sqrt{\frac{16\epsilon}{3\mulocaleps}+\frac{32 \sqrt{2\beta \epsilon}}{9 \sqrt{\mulocal m} M_{\mathrm{f}}}}  & k\geq k_0\\
        \enorm{\x_0 - \widehat{\xse}}- k \frac{\mulocal^{3/2}}{64 \beta^2 \sqrt{m} M_{\mathrm{f}}} & o.w.
    \end{cases}
\end{align*}
where $k_0 := \left\lceil \frac{4^4  \beta  \brac{\enorm{\x_0 - \widehat{\xse}} \frac{3\sqrt{m}\beta M_{\mathrm{f}}}{\sqrt{\mulocaleps }} -1} }{ 3\mulocaleps}\right\rceil$.
\end{proof}





% \section{OLD PAMOO proof}

% \begin{proof}
% Recall that for every $\w\in \reals^m_+$ it holds that $f_{\w}$ is a convex function. Hence, for every $\x,\y \in \reals^n$ it holds that
% \begin{align*}
%     &f_{\w}(\x) - f_{\w}(\y)  \leq \nabla f_\w(\x)^T(\x-\y). 
% \end{align*}
% Recall that the step size $\eta = 1$, then the update rule is given by $\x_{k+1} = \x_k - \nabla f_{\w_k}(\x_k)$. Then, for every $\x \in \reals^n$ we have
% \begin{align}
%     \enorm{\x_{k+1}-\x_\star}^2 &=\enorm{\x_k-\x_\star}^2 - 2\inner{\nabla f_{\w_k}(\x_k)}{\x_k - \x^*} + \enorm{\nabla f_{\w_k}(\x_k)}^2 \nonumber\\
%     &\leq \enorm{\x_k-\x_\star}^2 - 2 \brac{f_{\w_k}(\x_k)- f_{\w_k} (\x_\star)} +\enorm{\nabla f_{\w_k}(\x_k)}^2  \nonumber \\
%     & =\enorm{\x_k-\x_\star}^2 -  \max_{\w \in \reals_+^m} \Big{\{} 2\brac{f_{\w}(\x_k)- f_{\w} (\x_\star)} - \enorm{\nabla f_{\w}(\x_k)}^2 \Big{\}}, \label{eq:PAMOO_dist_from_opt}
% \end{align}
% where the last equality holds since $\w_k$ is the minimizer of this term  by the update rule of \texttt{PAMOO}, namely, 
% $$
% \w_k\in \argmax_{\w\in \reals^m_+} 2\brac{f_{\w_k}(\x_k)- f_{\w_k} (\x_\star)} - \enorm{\nabla f_{\w_k}(\x_k)}^2.
% $$
% Denote $\w_\star = \argmax\limits_{\w\in \Delta_{m,\wmin}} \lambda_{\min}\brac{\sum_{i=1}^m w_i \nabla^2 f_i(\x_\star)}$, $a_k = f_{\w_\star}(\x_k)- f_{\w_\star} (\x_\star)$, and $b_k = \enorm{\nabla f_{\w_\star}(\x_k)}^2$. Let $w(\x_k) = \w_\star \frac{a_k}{b_k} \in \reals^m_+$, we can lower bound of the last expression as follows
% \begin{align*}
%     \max_{\w\in \reals_+^m} \left[ 2\brac{f_{\w}(\x_k)- f_{\w} (\x_\star)} - \enorm{\nabla f_{\w}(\x_k)}^2 \right] & \geq 2\brac{f_{\w(\x_k)}(\x_k)- f_{\w(\x_k)} (\x_\star)}  -\enorm{\nabla f_{\w(\x_k)}(\x_k)}^2 \\
%     & =   \frac{\brac{f_{\w_\star}(\x_k)- f_{\w_\star} (\x_\star)}^2}{\enorm{\nabla f_{\w_\star}(\x_k)}^2}.
% \end{align*}
% Since $\w_\star\in \Delta_{m,\wmin}$ it holds that $f_{\w_\star}$ is $\beta$ smooth. Then, it holds that \textcolor{red}{YE: here we use the optimality of $\x_\star$. needs to be adapted to the approximate case} $\enorm{\nabla f_{\w_\star}(\x)}^2 \leq 2\beta \brac{f_{\w_\star}(\x)- f_{\w_\star} (\x_\star)}$ for every $\x$, and we have
% \begin{align*}
%      \max_{\w\in \reals_+^m} \left[ 2\brac{f_{\w}(\x_k)- f_{\w} (\x_\star)} - \enorm{\nabla f_{\w}(\x_k)}^2 \right] & \geq \frac{f_{\w_\star}(\x_k)- f_{\w_\star} (\x_\star)}{2 \beta} 
% \end{align*}
% Plugging this in Eq.~\eqref{eq:PAMOO_dist_from_opt}, we arrive to 
% \begin{align*}
%     \enorm{\x_{k+1}-\x_\star}^2 &\leq \enorm{\x_k-\x_\star}^2 -  \frac{ f_{\w_\star}(\x_k)- f_{\w_\star} (\x_\star)}{2 \beta}
% \end{align*}
% By Lemma~\ref{lemma:self_concordant} it holds that $f_{\w_\star}$ is $\widehat{M_{\mathrm{f}}}:=1/\sqrt{\wmin} M_{\mathrm{f}}$ self concordant. Then, From Lemma~\ref{lemma:self_con_consequences}, and its lower bound , i.e. $\omega\brac{t} \geq \frac{t^2}{2\brac{1+t}}$, we have
% \begin{align*}
%        f_{\w_\star}(\x_k) -f_{\w_\star}(\x_\star) \geq \inner{\nabla f_{\w_\star}(\x_\star)}{\x_k - \x_\star} +  \frac{\enorm{\x_k - \x_\star}_{ \x_\star,\w_\star}^2}{2\brac{1+\widehat{M_{\mathrm{f}}}\enorm{\x_k - \x_\star}_{\x_\star,\w_\star}}} = \frac{\enorm{\x_k - \x_\star}_{ \x_\star,\w_\star}^2}{2\brac{1+\widehat{M_{\mathrm{f}}}\enorm{\x_k - \x_\star}_{\x_\star,\w_\star}}}.
% \end{align*}
% The equality is due to the optimality condition, $\nabla f_i(\x_\star)=0$ for every $i \in [m]$, thus, $\nabla f_{\w_\star}(\x_\star) = \bold{0}$.
% Combining the last two equations, we have 
% \begin{align*}
%     \enorm{\x_{k+1}-\x_\star}^2 &\leq \enorm{\x_k-\x_\star}^2 -  \frac{1}{4 \beta} \frac{\enorm{\x_k - \x_\star}_{ \x_\star,\w_\star}^2}{1+\widehat{M_{\mathrm{f}}}\enorm{\x_k - \x_\star}_{\x_\star,\w_\star}}
% \end{align*}
% Note that $\lambda_{\min}\brac{\nabla^2 f_{\w_\star}(\x_\star)} \enorm{\x_\star - \x_k}^2 \leq \enorm{\x_\star - \x_k}_{\x_\star,\w_\star}^2 \leq \lambda_{\max}\brac{\nabla^2 f_{\w_\star}(\x_\star)} \enorm{\x_\star - \x_k}^2$. Since $\lambda_{\max}\brac{\nabla^2 f_{\w_\star}(\x_\star)} \leq \beta$ (smoothness), and since $w_{\min}= \mulocal /(8m\beta)$, then $\widehat{M_{\mathrm{f}}} \leq 3\sqrt{m\beta}M_{\mathrm{f}} /\sqrt{\mulocal}$. Thus, it holds that
% \begin{align*}
%     \enorm{\x_{k+1}-\x_\star}^2 &\leq \enorm{\x_k-\x_\star}^2 -  \frac{1}{4 \beta} \frac{\lambda_{\min}\brac{\nabla^2 f_{\w_\star}(\x_\star)} \enorm{\x_\star - \x_k}^2}{1+ \frac{3\sqrt{m} M_{\mathrm{f}} \beta}{\sqrt{\mulocal}}  \enorm{\x_k - \x_\star}}
% \end{align*}
% Using the assumption that $\max\limits_{\w\in \Delta_m}\lambda_{\min}\brac{\nabla^2 f_{\w}(\x_\star)} \geq \mulocal$, Lemma~\ref{lemma:mu_star_minimal_eigenvalue}, we have that
% \begin{align*}
%     \lambda_{\min} \brac{\nabla^2f_{\w_\star}(\x_\star)}\geq \max\limits_{\w\in \Delta_m}\lambda_{\min}\brac{\nabla^2 f_{\w}(\x_\star)} - 2m\wmin\beta \geq \mulocal - \mulocal/4 = (3/4)\mulocal.
% \end{align*}
% Finally, we obtain the recurring equation we wish:
% \begin{align*}
%     \enorm{\x_{k+1}-\x_\star}^2 &\leq \enorm{\x_k-\x_\star}^2 -  \frac{3 \mulocal}{16 \beta} \frac{ \enorm{\x_\star - \x_k}^2}{1+ \frac{3\sqrt{m} M_{\mathrm{f}} \beta}{\sqrt{\mulocal}}  \enorm{\x_k - \x_\star}}
% \end{align*} 
% Denote $\alpha_1 = \frac{3\mulocal}{16\beta}$, and $\alpha_2 = \frac{3\sqrt{m}\beta M_{\mathrm{f}}}{\sqrt{\mulocal}}$. Note that $\alpha_1 \in (0,1]$, $\alpha_2 \in \reals_+$, and $\enorm{\x-\x_\star} \in \reals_+$ for every $\x \in \reals^n$, we arrive to the recurrence relation analyzed in Lemma~\ref{lemma:iteration_bound}. Then, we obtain
% \begin{align*}
%     \enorm{\x_{k} - \x_\star} \leq 
%     \begin{cases}
%         \frac{\sqrt{\mulocal}}{3\sqrt{m}\beta M_{\mathrm{f}}} \brac{1-\frac{3\mulocal}{32\beta}}^{(k-k_0)/2}  & k\geq k_0\\
%         \enorm{\x_0 - \x_\star}- k \frac{\mulocal^{3/2}}{64 \beta^2 \sqrt{m} M_{\mathrm{f}}} & o.w.
%     \end{cases}
% \end{align*}
% where $k_0 := \left\lceil \frac{64 \beta  \brac{\enorm{\x_0 - \x_\star} 3\sqrt{m}\beta M_{\mathrm{f}} -\sqrt{\mulocal}} }{ 3\mulocal^{3/2}}\right\rceil$.
% \end{proof}









\section{Missing Proofs}\label{app:missing_proofs}

\subsection{Proof of Proposition ~\ref{prop:unique_optimal_sol}}\label{app:missing_proofs_unique_opt_sol}
Let us restate the claim:

\UniqueSol*

\begin{proof}
Let $\x_\star$ be a minimizer of all functions $\{ f_i\}_{i\in[m]}$ which exists due to the AMOO assumption, namely, a solution of 
\begin{align}
    \x_\star \in \argmin_{\x} f_i(\x)\ \forall i\in [m]. \label{eq:app_amoo_assumption}
\end{align}
 
By assumption, it holds that for the weight vector $\w_\star\in \argmax_{\w\in \Delta_m}\lambda_{\min}\left(\sum_{i=1}^m w_i \nabla^2 f_i(\x_\star) \right)$ it holds that $\lambda_{\min}\left(\sum_{i=1}^m \nabla^2 f_{\w_\star}(\x_\star) \right)>0$, namely,
\begin{align}
    \nabla^2 f_{\w_\star}(\x_\star) \succ 0. \label{eq:f_w_star_stictly_pos}
\end{align}
Notice that $\x_\star$ is a minimizer of $f_{\w_\star}$ (Lemma~\ref{lemma:optimality_of_x_star}), and that $f_{\w_\star}$ is a convex function, since $f_i$ are convex and $\w_\star$ has non-negative components. Combining with Eq.~\eqref{eq:f_w_star_stictly_pos}, it implies that $\x_\star$ is a unique minimizer of $f_{\w_\star}$.

Assume, by way of contradiction, there exists an additional minimizer that solves Eq.~\eqref{eq:app_amoo_assumption}, denote by $\widehat{\x}_\star.$ Since it is a solution of Eq.~\eqref{eq:app_amoo_assumption}, it is also a minimizer of $f_{\w_\star}$. This contradicts the fact $f_{\w_\star}$ has a unique optimal solution $\x_\star.$ 

\end{proof}


\subsection{Proof of Proposition~\ref{thm:app_hessian}}\label{app:weyls consequence}
The proof of Proposition~\ref{thm:app_hessian} is a corollary of Theorem~\ref{thm:weyls} (Weyl's Theorem). We establish the result for a general deviation in Hessian matrices without requiring it to be necessarily diagonal.

Let us restate the result:
\ApproxHessian*

\begin{proof}
    
Denote $\A_i := \nabla^2 f_i(\x) + \Delta_i$ for every $i\in [m]$, and $\sum_i^m \Delta_i = \Delta$. Let $\w_\star $, and $\hat{\w}_\star$ denote the solution of,
    \begin{align*}
        \w_\star \in \argmax_{\w\in \Delta} \lambda_{\min}\brac{\sum_i w_i \nabla^2 f_i(\x)}, ~~~~~ \text{and} ~~~~~~~ \hat{\w}_\star \in \argmax_{\w\in \Delta} \lambda_{\min}\brac{\sum_i w_i \A_i},
    \end{align*}
    respectively. Let $g(\w_\star)$, and $\hat{g}(\hat{\w}_\star)$ denote the optimal value, $g(\w_\star) = \lambda_{\min} \brac{\sum_i w_{\star, i}  \nabla^2 f_i(\x)}$, and $\hat{g}(\hat{\w}_\star) = \lambda_{\min} \brac{\sum_i \hat{w}_{\star, i} \A_i}$. Then, since $\hat{g}(\w_\star) -\hat{g}(\hat{\w}_\star)\leq 0$ by the optimality of $\hat{\w}_\star$ on $\hat{g}$, the following holds
    \begin{align*}
        g(\w_\star) & = g(\w_\star) - \hat{g}(\w_\star) + \hat{g}(\w_\star) -\hat{g}(\hat{\w}_\star) +\hat{g}(\hat{\w}_\star) - g(\hat{\w}_\star) +g(\hat{\w}_\star) \\
        & \leq |g(\w_\star) - \hat{g}(\w_\star)|  + |\hat{g}(\hat{\w}_\star) - g(\hat{\w}_\star)| +g(\hat{\w}_\star)\\
    \end{align*}
    Using Theorem~\ref{thm:weyls} (Weyl's Theorem) the followings are hold: $|g(\w_\star) - \hat{g}(\w_\star)| \leq \Delta$, and $|\hat{g}(\hat{\w}_\star) - g(\hat{\w}_\star)| \leq \Delta$. Then, we obtain 
    \begin{align*}
        g(\w_\star) & \leq 2\enorm{\Delta} +g(\hat{\w}_\star)
    \end{align*}
    Finally, since $g(\w_\star)\geq \muglobal$, by Definition~\ref{def:mu_global}, we obtain the proof.
\end{proof}


\subsection{Proof of Lemma~\ref{lemma:exact_iteration_bound}}\label{app:exact_iteration_bound_proof}
Let us restate the claim:

\ExactIterationBound*

\begin{proof}
We split the proof into two regimes, the incremental convergence and linear convergence regime.


\paragraph{Incremental convergence, $r_k> 1/\alpha_2$.} With this assumption we have $1+r_k \alpha_2 < 2 r_k \alpha_2$. Then, the following bound holds:
% {\color{blue} 
% \begin{align*}
%      r_{k+1}^2 &\leq r_k^2 \brac{1-\frac{\alpha_1}{2\alpha_2 r_k}}.
% \end{align*}
% Since $\alpha_1 \in (0,2)$, $\alpha_2 r_k> 1$ we have that $\frac{\alpha_1}{2 \alpha_2 r_k} \in(0,1)$. Thus, for every $k'<k$ the recursive equation is still in this convergence regime. Thus, for every $k'<k$ holds that $r_{k'}> 1/\alpha_2$, and we obtain that.
% \begin{align*}
%      r_{k+1}^2 &\leq r_k^2 \brac{1-\frac{\alpha_1}{2\alpha_2 r_0}} \leq r_0^2 \brac{1-\frac{\alpha_1}{2\alpha_2 r_0}}^k.
% \end{align*}
% By solving $\frac{1}{\alpha_2}^2 \geq r_0^2 \brac{1-\frac{\alpha_1}{2\alpha_2 r_0}}^{k_0}$ we conclude the maximal iteration after which $r_k \leq 1/\alpha_2$, namely, after at most $k_0$ iterates $r_k$ out from the first convergence regime.
% }
\begin{align*}
     r_{k+1} &\leq r_k\sqrt{1-\frac{\alpha_1}{2\alpha_2 r_k}}.
\end{align*}
Recall that $\sqrt{1-y}\leq 1-\frac{y}{2}$ for every $y \leq 1$. Since $ \frac{1}{\alpha_2 r_k}<  1$ we have $ \frac{\alpha_1}{2\alpha_2 r_k}<  \frac{\alpha_1}{2} < 1$.
Hence,
\begin{align*}
    r_{k+1} \leq r_k\brac{1-\frac{\alpha_1}{4\alpha_2 r_k}} = r_k - \frac{\alpha_1}{4\alpha_2}.
\end{align*}
For every $k'<k$ the recursive equation is still in the incremental convergence regime. Thus, for every $k'<k$ holds that $r_{k'}> 1/\alpha_2$.

By solving $1/\alpha_2 \geq r_0 - k_0\alpha_1/4\alpha_2$ we conclude the maximal iteration after which $r_k\leq 1/\alpha_2$, namely, after at most $k_0$ iterates $r_k$ out from the incremental convergence regime.

\paragraph{Linear convergence, $r_k\leq 1/\alpha_2$.} With this assumption we have the following bound on the recursive equation:
 \begin{align*}
     r_{k+1}^2 \leq \brac{1-\frac{\alpha_1}{2}}r_{k}^2.
 \end{align*}
Further, since for every $k'\geq k$ it holds that $r_{k'}\leq r_{k} \leq 1/\alpha_2 $ the recursive equation continues in the linear convergence regime. Thus, after at most $k_0$ iterations $r_k$ is in the linear convergence regime.

\end{proof}




\subsection{Proof of Lemma~\ref{lemma:epsilon_app_iteration_bound}}
Let us restate the claim:
\EpsilonIterationBound*
\begin{proof}
We split the proof into two regimes, the incremental convergence and linear convergence regime. 

 \paragraph{Incremental convergence, $r_k> 1/\alpha_2$.} With this assumption we have $1+r_k \alpha_2 < 2 r_k \alpha_2$. Then, the following bound holds:
 \begin{align*}
     r_{k+1} &\leq \sqrt{ r_k^2 -\frac{\alpha_1r_k}{2\alpha_2} + \alpha_4 r_k+\alpha_3}  = \sqrt{r_k^2 \brac{1 -\frac{\alpha_1- 2\alpha_2\alpha_4}{2\alpha_2 r_k}} +\alpha_3} \leq r_k\sqrt{1-\frac{\alpha_1}{4\alpha_2 r_k}} + \sqrt{\alpha_3}.
 \end{align*}
 The third relation holds since $\alpha_4\leq \frac{\alpha_1}{4\alpha_2}$ by assumption which implies $\alpha_1/2\geq 2 \alpha_2 \alpha_4$ and by $\sqrt{a+b}\leq \sqrt{a}+\sqrt{b}$ for $a,b\geq 0$. 
 
 Recall that $\sqrt{1-y}\leq 1-y/2$ for every $y \leq 1$. Since $ \frac{1}{\alpha_2 r_k}<  1$ we have $ \frac{\alpha_1}{2\alpha_2 r_k}<  \frac{\alpha_1}{2} < 1$. % by the concavity of the function at $y=0$
 Hence,
\begin{align*}
    r_{k+1} \leq r_k\brac{1-\frac{\alpha_1}{8\alpha_2 r_k}} +\sqrt{\alpha_3}= r_k - \frac{\alpha_1}{8\alpha_2} +\sqrt{\alpha_3} \leq r_k - \frac{\alpha_1}{16\alpha_2},
\end{align*}
since $\alpha_3 \leq \frac{\alpha_1^2}{256\alpha^2_2}= \frac{\alpha_1^2}{16^2\alpha^2_2} $ by assumption. For every $k'<k$ the recursive equation is still in the incremental convergence regime. Thus, for every $k'<k$ holds that $r_{k'}> 1/\alpha_2$.

By solving $1/\alpha_2 \geq r_0 - k_0\alpha_1/16\alpha_2$ we conclude the maximal iteration after which $r_k\leq 1/\alpha_2$, namely, after at most $k_0$ iterates $r_k$ out from the incremental convergence regime.

\paragraph{Linear convergence, $r_k\leq 1/\alpha_2$.} With this assumption we have the following bound on the recursive equation:
 \begin{align}
     r_{k+1}^2 \leq \brac{1-\frac{\alpha_1}{2}}r_{k}^2 +\alpha_3 +\alpha_4 /\alpha_2 = \brac{1-\frac{\alpha_1}{2}}r_{k}^2 +\alpha', \label{eq:recursion bound induction}
 \end{align}
 where $\alpha':=\alpha_3 +\alpha_4 /\alpha_2.$
We will first show that $r_{k'}\leq 1/\alpha_2$ for all $k'\geq k.$ Observe that 
\begin{align*}
    r_{k+1}^2\leq \brac{1-\frac{\alpha_1}{2}}\frac{1}{\alpha_2^2} +\alpha' \leq \frac{1}{\alpha_2^2}
\end{align*}
since $ \alpha' = \alpha_3 +\frac{\alpha_4}{\alpha_2} \leq \frac{\alpha_1}{2\alpha^2_2}$ by assumption and by the fact $\alpha_1 \in (0,2)$. Hence, $r_{k+1}\leq \frac{1}{\alpha_2}$ which inductively implies that  $r_{k'}\leq r_k \leq 1/\alpha_2$ for all $k'\geq k \geq k_0$.

Since in this regime, for all $k'\geq k$ Eq.~\eqref{eq:recursion bound induction} holds, we can upper bound the recursive relation by
\begin{align*}
    r_{k'}^2 &\leq \brac{1-\frac{\alpha_1}{2}}^{k'-k} 
    r_k^2 + \sum_{t=0}^\infty \brac{1-\frac{\alpha_1}{2}}^t \alpha' \leq r_{k_0}^2 \brac{1-\frac{\alpha_1}{2}}^{k'-k} + \frac{2\alpha'}{\alpha_1}
\end{align*}
where the last inequality holds by summing the geometric series and since $1-\alpha_1/2\in (0,1).$ This inequality implies the result
since
\begin{align*}
    r_{k'}\leq r_{k_0} \brac{1-\frac{\alpha_1}{2}}^{\frac{k'-k}{2}} + \sqrt{\frac{2\alpha'}{\alpha_1}} = r_{k_0} \brac{1-\frac{\alpha_1}{2}}^{\frac{k'-k}{2}} + \sqrt{\frac{2\alpha_3}{\alpha_1}+\frac{2\alpha_4}{\alpha_1 \alpha_2}}
\end{align*}
by $\sqrt{a+b}\leq \sqrt{a}+\sqrt{b}$ for $a,b\geq 0$. Finally, since for every $k'\geq k$ it holds that $r_{k'}\leq r_{k} \leq 1/\alpha_2 $ the recursive equation continues in the linear convergence regime. Thus, after at most $k_0$ iterations $r_k$ is in the linear convergence regime.


\end{proof}



\subsection{Proof of Lemma~\ref{lemma:wmin_minimal_eigenvalue}}
Let us restate the claim:
\ContOfMinEigenOfHessian*

\begin{proof}
        To establish the lemma we want to show that for any $\w\in \Delta_{m}$ there exists $\widehat{\w}\in \Delta_{m,\wmin}$ such that $\lambda_{\min} \brac{\sum_{i} \hat{w}_i \nabla^2 f_i(\x)}\geq \lambda_{\min} \brac{\sum_{i} w_i \nabla^2 f_i(\x)}-2m\wmin\beta$. We start by bounding the following term $\enorm{\nabla^2 f_\w(\x) - \nabla^2 f_{\hat{\w}}(\x)}_2$ for any $\x\in \reals^n$. By the triangle inequality and the positive homogeneity, we have 
    \begin{align*}
       &\enorm{\sum_i(w_i-\hat{w}_i)\nabla^2 f_i(\x)}_2 \leq  \sum_i \enorm{(w_i-\hat{w}_i) \nabla^2 f_i(\x)}_2 = \sum_i |w_i-\hat{w_i}|\enorm{ \nabla^2 f_i(\x)}_2  \leq \beta \sum_i |w_i-\hat{w_i}|,
    \end{align*}
    while the last inequality holds since $\{f_i\}_{i\in[m]}$ are $\beta$ smooth. Since for any $\w\in \Delta_m$ there exist $\hat{\w}\in \Delta_{m,\wmin}$ such that $\sum_i |w_i-\hat{w_i}| \leq 2m\wmin$, we obtain that for every $\x\in\reals^n$ it holds that 
    \begin{align*}
       &\enorm{\nabla^2 f_\w(\x) - \nabla^2 f_{\hat{\w}}(\x)}_2 = \enorm{\sum_i(w_i-\hat{w}_i)\nabla^2 f_i(\x)}_2 \leq  2m\wmin\beta.
    \end{align*}
    Thus, by using Theorem~\ref{thm:weyls} we obtain that for any $\w\in \Delta_m$
    \begin{align*}
         | \lambda_{\min} (\nabla^2 f_\w(\x)) - \lambda_{\min} (\nabla^2 f_{\hat{\w}}(\x)) | \leq \enorm{\nabla^2 f_\w(\x) - \nabla^2 f_{\hat{\w}}(\x)}_2 \leq  2m\wmin\beta.
    \end{align*}
    By setting $\w$ as $\w_\star$ we conclude the result.
\end{proof}




% \begin{table}[t]
% \centering
% \renewcommand{\arraystretch}{1.25}  % Increases row height
% \begin{tabular}{|>{\centering\arraybackslash}p{3.2cm}|>{\centering\arraybackslash}p{4.5cm}|}
% \hline
% \rowcolor{gray!50} \makecell{Algorithm} & \makecell{Asymptotic Convergence} \\
% \hline
%  \makecell{Equal weights} & $O\brac{\brac{1- \frac{\muglobal}{m\beta}}^{k}}$ \\
% \hline
%  \makecell{CAMOO} & $O\brac{\brac{1-\frac{\muglobal}{\beta}}^{k}}$ \\
% \hline
%  \makecell{PAMOO} &  $O\brac{\brac{1-\frac{\mulocal}{\beta}}^{k}}$  \\
% % \hline
% % \makecell{Equal Weights (\texttt{EW})} & $\Omega\brac{1-\muglobal/m\beta}^{k}$  \\
% \hline
% \end{tabular}
% \caption{
% }
% \end{table}




%%% OLD ONE
% \newpage

% \section{Proofs of Theoretical Results} \label{app:theory}
% {\color{red} BK: the section is an old one!}
% \subsection{Preliminaries and Basic Properties} \label{app:preliminaries}
% % TODOs: add proper continuouty assumptions?

% In this section, we formally provide our working assumptions. We assume access to multi-objective feedback with $m$ objectives $F(\x) = (f_1(\x),\ldots,f_m(\x))$. Considering AMOO, we assume the functions are aligned in the sense of Eq.~\eqref{eq:aligned_functions}, namely, that they share an optimal solution. 

% We define the following quantities, for the single and multi objective settings:
% \begin{align*}
%     &\enorm{\y}^2_{\x}:=\enorm{\y}_{\nabla^2 f(\x)} := \langle \nabla^2 f(\x) \y, \y \rangle \\
%     &\enorm{\y}^2_{\x,\w} :=\enorm{\y}_{\nabla^2 f_\w(\x)} := \langle \nabla^2 f_\w(\x) \y, \y \rangle.
% \end{align*}

% % \begin{assumption}[Locally Optimal Curvature] \label{ass:mu_star}
% %     For any $\x\in \mX$ there exist a weight vector $\w\in \Delta_m$ such that  
% %     \begin{align}
% %        \lambda_{\min}\left(\sum_{i=1}^m w_i \nabla^2 f_i(\x) \right)\geq \muglobal. \nonumber
% %     \end{align}
% % \end{assumption}


% \begin{assumption}[Smoothness] \label{ass:smooth}
%     All function are $\beta$-smooth. $\forall i\in [m]$, $f_i: \reals^n \xrightarrow{} \reals$ it holds that $~\forall \x, \y \in \reals^n$:
%     \begin{align}
%         f(\y) \leq  f(\x) + \nabla f(\x)^{\top} (\y - \x) + \frac{\beta}{2}  \enorm{ \x - \y } ^2. \nonumber
%     \end{align}
% \end{assumption}
% \begin{assumption}[Self-concordant] \label{ass:self_con}
%     All functions are self-concordant with $M_{\mathrm{f}} \geq 0$ parameter.  $\forall i\in [m]$  $f: \reals^n \xrightarrow{} \reals$ and $~\forall \x,\y\in \reals^n$:
%     \begin{align}
%         \inner{\nabla^3 f_i(\x)[\y]\y}{\y}  \preceq 2M_{\mathrm{f}} \enorm{\y}_{\x}^3, \nonumber
%     \end{align}
%     where $\nabla^3 g(\x)[\y] := \lim_{\alpha\rightarrow 0} \frac{1}{\alpha}\brac{\frac{\nabla^2 g(\x+\alpha \y) - \nabla^2 g(\x)}{\alpha}}$ is the directional derivative of the hessian in~$\y$.
% \end{assumption}


% These assumptions have the following important consequences.

% \begin{lemma}[Theorem 5.1.8 \& Lemma 5.1.5,~\citet{nesterov2013introductory}]\label{lemma:self_con_consequences}
% Let $f:\reals^n \rightarrow \reals$ be an $M_{\mathrm{f}}$ self-concordant function. Let $x, y\in\reals^n$ , we have
% $$
% f(\y) \geq f(\x) + \inner{\nabla f(\x)}{\y  - \x} + \frac{1}{M_{\mathrm{f}}^2} \omega\brac{M_{\mathrm{f}}\enorm{\y-\x}_\x },
% $$
% where $\omega(t) := t-\ln(1-t)$, and, for any $t>0$, $\omega(t)\geq \frac{t^2}{2(1+t)}$.
% \end{lemma}
% \begin{lemma}[Theorem 5.1.1, ~\citet{nesterov2018lectures}]\label{lemma:sum_of_self_con}
%     Let $f_1,f_2 : \reals^n \to \reals$ be $M_{\mathrm{f}}$ self-concordant functions. Let $w_1,w_2 > 0$. Then, $f=w_1 f_1+ w_2 f_2$ is $M = \max_i \{ \frac{1}{\sqrt{w_i}} \} M_{\mathrm{f}}$ self-concordant function.
% \end{lemma}
% \begin{restatable}[Weighted sum of self-concordant functions]{proposition}{SumSelfCon} \label{prop:sun_of_self_con}
%     Let $\{ f_i: \reals^n \to \reals \}_{i=1}^{n} $ be $M_{\mathrm{f}}$ self-concordant functions. Let $\{w_i > 0\}$. Then, $f= \sum_{i=1}^{n} w_i f_i$ is $M = \max_i \{ \frac{1}{\sqrt{w_i}} \} M_{\mathrm{f}}$ self-concordant function.
% \end{restatable}
% \begin{lemma}[Standard result, E.g., 9.17~\citet{boyd2004convex}] \label{lemma:smooth-gradient-norm}
%     Let $f : \reals^n \to \reals$ a $\beta$-smooth over $\reals^n$, and let $\x_\star \in \arg\min_{\x} ~ f(\x)$.  Then, it holds that
%     \begin{align*}
%         \enorm{\nabla f (\x)}^2 \leq 2\beta \brac{f(\x) - f(\x_\star)}.
%     \end{align*}
% \end{lemma}
% \begin{theorem}[Weyl's Theorem]\label{thm:weyls} Let $\A$ and $\Delta$ be symmetric matrices in $\reals^{d\times d}$. Let $\lambda_j(\A)$ be the jth largest eigenvalue of a matrix $\A$. Then, for all $j\in [d]$ it holds that $\| \lambda_j(\A) - \lambda_j(\A+\Delta) \| \leq \| \Delta\|_2$, where $\| \Delta\|_2$ is the operator norm of $\Delta$.
% \end{theorem}



% Further, we have the following simple consequence of the AMOO setting.
% \begin{lemma}\label{lemma:optimality_of_x_star}
% For all $\w\in \Delta_m$ and $\x\in \reals^n$ it holds that $f_\w(\x) - f_\w(\x_\star)\geq 0.$
% \end{lemma}
% % \begin{proof}
% %     By using optimality of $\x_\star$, and smoothness of $f(\cdot)$ (Def.\ref{def:smooth}), for every $\y, \x \in \mX$ it holds that 
% %     \begin{align*}
% %         f(\x_\star) \leq f(\y) \leq f(\x) + \nabla f(\x)^\top \brac{\y-\x} + \frac{\beta}{2} \enorm{\y-\x}^2 \\
% %     \end{align*}
% %     Since $\y = \x - \eta \nabla f(\x)$. We have
% %     \begin{align*}
% %         f(\x_\star)  \leq f(\x) -\eta \enorm{\nabla f(\x)}^2 + \frac{\beta}{2} \eta^2 \enorm{\nabla f(\x)}^2 =  f(\x) - \eta \enorm{\nabla f(\x)}^2 \brac{ 1 - \frac{\beta \eta}{2}  }
% %     \end{align*}
% %     Plugging in $\eta = \beta^{-1}$, we obtain that
% %     \begin{align*}
% %         f(\x_\star) \leq f(\x) - \frac{\eta}{2} \enorm{\nabla f(\x)}^2 
% %     \end{align*}
% % \end{proof}
% % {\color{blue} add lemma that shows that the weighted function is smooth}
% \begin{proof}

%     Observe that
%     $
%         f_\w(\x) - f_\w(\x_\star)= \sum_{i=1}^m w_i \brac{f_i(\x) - f_i(\x_\star)}.
%     $
%     Since $\x_\star$ is the optimal solution for all objectives it holds that $f_i(\x) - f_i(\x_\star) \geq  0.$ The lemma follows from the fact $w_i\geq 0$ for all $i\in [m].$
% \end{proof}

% % Further, recall the following observation holds.
% % \begin{observation}\label{obs:simplex_sum}
% %     Let $\w \in \Delta_m$. Assume $\{ f_i \}_{i=1}^m$ are  $ \beta $ smooth and $M_{\mathrm{f}}$ self-concordant. Then, $f_{\w}(\x) := \sum_{i=1}^{m} w_i f_i(\x)$ is also $\beta$ smooth and $M_{\mathrm{f}}$ self-concordant.
% % \end{observation} 

% % OLDER RECURRENCE
% % \begin{lemma}[Recurrence bound]\label{lemma:iteration_bound}
% % Let $\{ x_k\}_{k\geq 0}$ be a sequence of non-negative real numbers that satisfy the recurrence relation
% % \begin{align*}
% %     x_{k+1}^2 \leq x_k^2 -\alpha_1\frac{x_k^2}{1+ \alpha_2 x_k},
% % \end{align*}
% % where $\alpha_1\in [0,2)$ and $\alpha_2\in \reals_+.$ Then, $x_k$ is bounded by
% %     \begin{align*}
% %         x_k \leq 
% %         \begin{cases}
% %             \brac{1-\alpha_1/2}^{(k-k_0)/2} / \alpha_2 & k\geq k_0\\
% %             x_0 - k \alpha_1/4\alpha_2 & o.w.
% %         \end{cases}
% %     \end{align*}
% % where $k_0 := \lceil 4 / \alpha_1 \brac{x_0 \alpha_2 - 1}\rceil.$
% % \end{lemma}

% % \begin{proof}
% % We split the proof into two regimes, the linear convergence and incremental convergence regime.

% % \paragraph{Linear convergence, $x_k\leq 1/\alpha_2$.} With this assumption we have the following bound on the recursive equation:
% %  \begin{align*}
% %      x_{k+1}^2 \leq \brac{1-\frac{\alpha_1}{2}}x_{k}^2.
% %  \end{align*}
% % Further, since for every $k'\geq k$ it holds that $x_{k'}\leq x_{k} \leq 1/\alpha_2 $ the recursive equation continues in the linear convergence regime.

% %  \paragraph{Incremental convergence, $x_k> 1/\alpha_2$.} With this assumption we have $1+x_k \alpha_2 < 2 x_k \alpha_2$. Then, the following bound holds:
% %  \begin{align*}
% %      x_{k+1} &\leq x_k\sqrt{1-\frac{\alpha_1}{2\alpha_2 x_k}}.
% %  \end{align*}
% %  Recall that $\sqrt{1-y}\leq 1-y/2$ for every $y \leq 1$. Since $ \frac{1}{\alpha_2 x_k}<  1$ we have $ \frac{\alpha_1}{2\alpha_2 x_k}<  \frac{\alpha_1}{2} < 1$. % by the concavity of the function at $y=0$
% %  Hence,
% % \begin{align*}
% %     x_{k+1} \leq x_k\brac{1-\frac{\alpha_1}{4\alpha_2 x_k}} = x_k - \frac{\alpha_1}{4\alpha_2}.
% % \end{align*}
% % For every $k'<k$ the recursive equation is still in the incremental convergence regime. Thus, for every $k'<k$ holds that $x_{k'}> 1/\alpha_2$.

% % Finally, by solving $1/\alpha_2 = x_0 - k_0\alpha_1/4\alpha_2$ we conclude the maximal iteration after which $x_k\leq 1/\alpha_2$, namely, after at most $k_0$ iterates $x_k$ exhibits linear convergence.
% % \end{proof}

% % \textcolor{red}{YE: TODO: change to $r_k$ from $x_k$, since $r$ is residual.}

% \begin{lemma}[Recurrence bound]\label{lemma:iteration_bound}
% Let $\{ r_k\}_{k\geq 0}$ be a sequence of non-negative real numbers that satisfy the recurrence relation
% \begin{align*}
%     r_{k+1}^2 \leq r_k^2 -\alpha_1\frac{r_k^2}{1+ \alpha_2 r_k} +\alpha_3 +\alpha_4 r_k,
% \end{align*}
% where $\alpha_1\in (0,2)$, $\alpha_2\in \reals_+,$ $\alpha_3 \leq \frac{\alpha_1^2}{256\alpha^2_2},$ and $\alpha_4\leq \frac{\alpha_1}{4\alpha_2}.$ Then, $r_k$ is bounded by
%     \begin{align*}
%         r_k \leq 
%         \begin{cases}
%             \brac{1-\alpha_1/2}^{(k-k_0)/2} / \alpha_2 +\sqrt{ 2\alpha_3/\alpha_1 +\alpha_4 /\brac{\alpha_2\alpha_1}} & k\geq k_0\\
%             r_0 - k \alpha_1/16\alpha_2 & o.w.
%         \end{cases}
%     \end{align*}
% where $k_0 := \lceil 8 / \alpha_1 \brac{r_0 \alpha_2 - 1}\rceil.$
% \end{lemma}

% \begin{proof}
% We split the proof into two regimes, the linear convergence and incremental convergence regime. \textcolor{red}{YE: verify it makes sense! (might be numerical errors)}{\color{blue} BK: Now, there are no numerical errors! I believe that the "Incremental convergence" is not tight, i.e. we can show linear convergence with different rates for both cases. I will try it after finishing with PAMOO}

% \paragraph{Linear convergence, $r_k\leq 1/\alpha_2$.} With this assumption we have the following bound on the recursive equation:
%  \begin{align}
%      r_{k+1}^2 \leq \brac{1-\frac{\alpha_1}{2}}r_{k}^2 +\alpha_3 +\alpha_4 /\alpha_2 = \brac{1-\frac{\alpha_1}{2}}r_{k}^2 +\alpha', \label{eq:recursion bound induction}
%  \end{align}
%  where $\alpha':=\alpha_3 +\alpha_4 /\alpha_2.$
% We will first show that $r_{k'}\leq 1/\alpha_2$ for all $k'\geq k.$ Observe that 
% \begin{align*}
%     r_{k+1}^2\leq \brac{1-\frac{\alpha_1}{2}}\frac{1}{\alpha_2^2} +\alpha' \leq \frac{1}{\alpha_2^2}
% \end{align*}
% since 
% $$
% \alpha' = \alpha_3 +\frac{\alpha_4}{\alpha_2} \leq \frac{\alpha_1^2}{256\alpha^2_2} +\frac{\alpha_1}{4\alpha_2^2} =\frac{(\alpha_1/2)^2}{64\alpha^2_2} +\frac{\alpha_1}{4\alpha_2^2} \leq \frac{\alpha_1/2}{64\alpha^2_2} +\frac{\alpha_1}{4\alpha_2^2} \leq \frac{\alpha_1}{2\alpha^2_2}
% $$
% by assumption and by the fact $\alpha_1 \in (0,2)$. Hence, $r_{k+1}\leq \frac{1}{\alpha_2}$ which inductively implies that  $r_{k'}\leq 1/\alpha_2$ for all $k'\geq k.$

% Since in this regime, for all $k'\geq k$ Eq.~\eqref{eq:recursion bound induction} holds, we can upper bound the recursive relation by
% \begin{align*}
%     r_{k'}^2 &\leq \brac{1-\alpha_1/2}^{k'-k} x^2_k + \sum_{t=0}^\infty \brac{1-\alpha_1/2}^t \alpha'\\
%     &\leq \brac{1-\alpha_1/2}^{k'-k}/\alpha_2^2 + 2\alpha'/\alpha_1\\
% \end{align*}
% where the last inequality holds by summing the geometric series and since $1-\alpha_1/2\in (0,1).$ This inequality implies the result
% since
% \begin{align*}
%     r_{k'}\leq \brac{1-\alpha_1/2}^{(k'-k)/2}/\alpha_2 +\sqrt{2\alpha'/\alpha_1} = \brac{1-\alpha_1/2}^{(k'-k)/2}/\alpha_2 +\sqrt{ 2\alpha_3/\alpha_1 +\alpha_4 /\brac{\alpha_2\alpha_1}}
% \end{align*}
% by $\sqrt{a+b}\leq \sqrt{a}+\sqrt{b}$ for $a,b\geq 0.$

%  \paragraph{Incremental convergence, $r_k> 1/\alpha_2$.} With this assumption we have $1+r_k \alpha_2 < 2 r_k \alpha_2$. Then, the following bound holds:
%  \begin{align*}
%      r_{k+1} &\leq \sqrt{ r_k^2 -\frac{\alpha_1r_k}{2\alpha_2} + \alpha_4 r_k+\alpha_3} \\
%      & = \sqrt{r_k^2 \brac{1 -\frac{\alpha_1- 2\alpha_2\alpha_4}{2\alpha_2 r_k}} +\alpha_3}\\
%      &\leq r_k\sqrt{1-\frac{\alpha_1}{4\alpha_2 r_k}} + \sqrt{\alpha_3}.
%  \end{align*}
%  The third relation holds since $\alpha_4\leq \frac{\alpha_1}{4\alpha_2}$ by assumption which implies $\alpha_1/2\geq 2 \alpha_2 \alpha_4$ and by $\sqrt{a+b}\leq \sqrt{a}+\sqrt{b}$ for $a,b\geq 0$. 
 
%  Recall that $\sqrt{1-y}\leq 1-y/2$ for every $y \leq 1$. Since $ \frac{1}{\alpha_2 r_k}<  1$ we have $ \frac{\alpha_1}{2\alpha_2 r_k}<  \frac{\alpha_1}{2} < 1$. % by the concavity of the function at $y=0$
%  Hence,
% \begin{align*}
%     r_{k+1} \leq r_k\brac{1-\frac{\alpha_1}{8\alpha_2 r_k}} +\sqrt{\alpha_3}= r_k - \frac{\alpha_1}{8\alpha_2} +\sqrt{\alpha_3} \leq r_k - \frac{\alpha_1}{16\alpha_2},
% \end{align*}
% since $\alpha_3 \leq \frac{\alpha_1^2}{256\alpha^2_2}= \frac{\alpha_1^2}{16^2\alpha^2_2} $ by assumption. For every $k'<k$ the recursive equation is still in the incremental convergence regime. Thus, for every $k'<k$ holds that $r_{k'}> 1/\alpha_2$.

% Finally, by solving $1/\alpha_2 = r_0 - k_0\alpha_1/16\alpha_2$ we conclude the maximal iteration after which $r_k\leq 1/\alpha_2$, namely, after at most $k_0$ iterates $r_k$ exhibits linear convergence.
% \end{proof}


% \subsection{Proof of Proposition~\ref{prop:unique_optimal_sol}}\label{app:proof unique solution}

% Let us restate the claim:
% \UniqueSol*

% \begin{proof}
% Let $\x_\star$ be a minimizer of all functions $\{ f_i\}_{i\in[m]}$ which exists due to the AMOO assumption, namely, a solution of 
% \begin{align}
%     \x_\star \in \argmin_{\x} f_i(\x)\ \forall i\in [m]. \label{eq:app_amoo_assumption}
% \end{align}
 
% By assumption, it holds that for the weight vector $\w_\star\in \argmax_{\w\in \Delta_m}\lambda_{\min}\left(\sum_{i=1}^m w_i \nabla^2 f_i(\x_\star) \right)$ it holds that $\lambda_{\min}\left(\sum_{i=1}^m \nabla^2 f_{\w_\star}(\x_\star) \right)>0$, namely,
% \begin{align}
%     \nabla^2 f_{\w_\star}(\x_\star) \succ 0. \label{eq:f_w_star_stictly_pos}
% \end{align}
% Notice that $\x_\star$ is a minimizer of $f_{\w_\star}$ (Lemma~\ref{lemma:optimality_of_x_star}), and that $f_{\w_\star}$ is a convex function, since $f_i$ are convex and $\w_\star$ has non-negative components. Combining with Eq.~\eqref{eq:f_w_star_stictly_pos}, it implies that $\x_\star$ is a unique minimizer of $f_{\w_\star}$.

% Assume, by way of contradiction, there exists an additional minimizer that solves Eq.~\eqref{eq:app_amoo_assumption}, denote by $\widehat{\x}_\star.$ Since it is a solution of Eq.~\eqref{eq:app_amoo_assumption}, it is also a minimizer of $f_{\w_\star}$. This contradicts the fact $f_{\w_\star}$ has a unique optimal solution $\x_\star.$ 

% \end{proof}
    
% \subsection{Proof of Theorem~\ref{thm:exact_amoo_convergence}}\label{app:camoo}


% At a high level, the proof follows the standard convergence analysis of $\mu$-strongly convex and $L$-smooth function, while applying Lemma~\ref{lemma:self_con_consequences}, instead of using only properties of strongly convex functions alone.

% In addition, we choose the minimal weight value, $\wmin$, such that the weighted function at each iteration $f_{\w_k}$ has a sufficiently large self-concordant parameter, while the minimal eigenvalue of its Hessian is close to $\mu_\star$. Before proving Theorem~\ref{thm:exact_amoo_convergence}, we provide two results that allow us to control these two aspects.
% \begin{lemma}\label{lemma:self_concordant}
% For any iteration $t$, the function $f_{\w_k}$ is $1/\sqrt{\wmin}M_{\mathrm{f}}$ self-concordant.    
% \end{lemma}
% \begin{proof}
%     This is a direct consequence of Proposition~\ref{prop:sun_of_self_con} and the fact Algorithm~\ref{alg:AMOOO} sets the weights by optimizing over a set where the weight vector is lower bounded by $\wmin$.
% \end{proof}
% \begin{lemma}\label{lemma:mu_star_minimal_eigenvalue}
% Let $t\in[T]$, $\w \in \argmax\limits_{\w\in \Delta_{m}} \lambda_{\min} \brac{\sum_{i} w_i \nabla^2 f_i(\x_{k})}$, $\w_k \in \argmax\limits_{\w\in \Delta_{m,\wmin}} \lambda_{\min} \brac{\sum_{i} w_i \nabla^2 f_i(\x_{k})}$. It holds that $\lambda_{\min}\brac{\nabla^2f_{\w_k}}\geq \lambda_{\min}\brac{\nabla^2f_{\w}} - 2m\wmin\beta$.
% \end{lemma}




% \begin{proof}
%     % We establish this result by comparing the solutions of the two optimization problems:
%     % \begin{align*}
%     %      &(\mathrm{P1})\ \max_{\w\in \Delta_{m}} \lambda_{\min} \brac{\sum_{i} w_i \nabla^2 f_i(\x_{k})},\\
%     %      &(\mathrm{P2})\ \max_{\w\in \Delta_{m,\wmin}} \lambda_{\min} \brac{\sum_{i} w_i \nabla^2 f_i(\x_{k})}.
%     % \end{align*}
%     % Observe that $(\mathrm{P2})$ is a solution to the same optimization problem as $(\mathrm{P1})$ on a more constraint set, namely $ \Delta_{m,\wmin}\subseteq  \Delta_{m}.$ 

%     To establish the lemma we want to show that for any $\w\in \Delta_{m}$ there exists $\widehat{\w}\in \Delta_{m,\wmin}$ such that $\lambda_{\min} \brac{\sum_{i} \hat{w}_i \nabla^2 f_i(\x_{k})}\geq \lambda_{\min} \brac{\sum_{i} w_i \nabla^2 f_i(\x_{k})}-2m\wmin\beta$. We start by bounding the following term $\enorm{\nabla^2 f_\w(\x) - \nabla^2 f_{\hat{\w}}(\x)}_2$ for any $\x\in \reals^n$. By the triangle inequality and the positive homogeneity, we have 
%     \begin{align*}
%        &\enorm{\sum_i(w_i-\hat{w}_i)\nabla^2 f_i(\x)}_2 \leq  \sum_i \enorm{(w_i-\hat{w}_i) \nabla^2 f_i(\x)}_2 = \sum_i |w_i-\hat{w_i}|\enorm{ \nabla^2 f_i(\x)}_2  \leq \beta \sum_i |w_i-\hat{w_i}|,
%     \end{align*}
%     while the last inequality holds since $\{f_i\}_{i\in[m]}$ are $\beta$ smooth. Since for any $\w\in \Delta_m$ there exist $\hat{\w}\in \Delta_{m,\wmin}$ such that $\sum_i |w_i-\hat{w_i}| \leq 2m\wmin$, we obtain that for every $\x\in\reals^n$ it holds that 
%     \begin{align*}
%        &\enorm{\nabla^2 f_\w(\x) - \nabla^2 f_{\hat{\w}}(\x)}_2 = \enorm{\sum_i(w_i-\hat{w}_i)\nabla^2 f_i(\x)}_2 \leq  2m\wmin\beta.
%     \end{align*}
%     Thus, by using Theorem~\ref{thm:weyls} we obtain 
%     \begin{align*}
%          | \lambda_{\min} (\nabla^2 f_\w(\x)) - \lambda_{\min} (\nabla^2 f_{\hat{\w}}(\x)) | \leq \enorm{\nabla^2 f_\w(\x) - \nabla^2 f_{\hat{\w}}(\x)}_2 \leq  2m\wmin\beta.
%     \end{align*}
    
%     % {\color{blue} BK: (Is it OK to delete all of this?) To establish the lemma we want to show that for any $\w\in \Delta_{m}$ there exists $\hat{w}\in \Delta_{m,\wmin}$ such that $\lambda_{\min} \brac{\sum_{i} \hat{w}_i \nabla^2 f_i(\x_{k})}\geq \lambda_{\min} \brac{\sum_{i} w_i \nabla^2 f_i(\x_{k})}-\wmin\beta$. This implies the claim since
%     % \begin{align*}
%     %     &\max_{\w\in \Delta_{m}} \lambda_{\min} \brac{\sum_{i} w_i \nabla^2 f_i(\x_{k})}
%     %     = \lambda_{\min} \brac{\sum_{i} w^\star_i \nabla^2 f_i(\x_{k})}
%     %     \geq \lambda_{\min} \brac{\sum_{i} \hat{w}^\star_i \nabla^2 f_i(\x_{k})}- 2m\wmin\beta,
%     % \end{align*}
%     % for some $\hat{w}^\star\in  \Delta_{m,\wmin} - \wmin\beta$.

%     % We now prove the claim. Observe that for any $\w\in \Delta_m$ there exist $\hat{\w}\in \Delta_{m,\wmin}$ such that $\enorm{\w-\hat{\w}}_1\leq 2m\wmin.$ With this we bound $\enorm{\nabla^2 f_\w(\x) - \nabla^2 f_{\hat{\w}}(\x)}_2$ for any $\x$.
%     % \begin{align*}
%     %    &\enorm{\sum_i(w_i-\hat{w}_i)\nabla^2 f_i(\x)}_2\stackrel{(1)}{\leq} \sum_i |w_i-\hat{w_i}|\enorm{\nabla^2 f_i(\x)}_2\stackrel{(2)}{\leq} \beta \sum_i |w_i-\hat{w_i}|= 2m\wmin\beta,
%     % \end{align*}
%     % where $(1)$ holds since $ f_i(\x)$ are $\beta$ smooth and, hence, the maximal eigenvalue of their Hessian is bounded by $\beta,$ and $(2)$, holds since $\enorm{\w-\hat{\w}}_1\leq 2M\wmin.$ Applying Proposition~\ref{thm:app_hessian} (a variation of Weyl's Theorem) implies the result we wanted to show. \textcolor{red}{TODO: prove}.}
% \end{proof}
% With these two results, we are ready to prove Theorem~\ref{thm:exact_amoo_convergence} which we restate:
% \ExactAmooConvergence*

% \begin{proof}
% At each iteration Algorithm~\ref{alg:Weighted-GD} gets $\w_k \in\argmax\limits_{\w\in \Delta_{m,w_{\min}}} \lambda_{\min} \brac{\sum_{i} w_i \nabla^2 f_i(\x_{k})}$. Using the assumption that $\max\limits_{\w\in \Delta_m}\lambda_{\min}\brac{\nabla^2 f_{\w_k}(\x_k)} \geq \muglobal$, Lemma~\ref{lemma:mu_star_minimal_eigenvalue}, and since we set $w_{\min}=\muglobal/\brac{8m\beta}$ we have that
% \begin{align}
%     \lambda_{\min} \brac{\nabla^2f_{\w_k}}\geq \lambda_{\min}\brac{\nabla^2f_{\w}} - 2m\wmin\beta \geq \muglobal - \muglobal/4 = (3/4)\muglobal , \label{eq:strongly_convex_param_of_AMOOO}
% \end{align}
% for all iterations $t$.
% Recall that the update rule is given by $\x_{k+1} = \x_k - \eta\nabla f_{\w_k}(\x_k)$, where $\eta$ is the step size.
% Then, for every $\x \in \reals^n$ we have
% \begin{align}
%     \enorm{\x_{k+1}-\x}^2 &= \enorm{\x_k-\eta\nabla f_{\w_k}(\x_k)-\x}^2 \nonumber \\
%     &=\enorm{\x_k-\x}^2 - 2\eta\inner{\nabla f_{\w_k}(\x_k)}{\x_k - \x} + \eta^2\enorm{\nabla f_{\w_k}(\x_k)}^2 \label{eq:camoo_gd_recursion}.
% \end{align}
% By Lemma~\ref{lemma:self_concordant} it holds that $f_{\w_k}$ is 
% \begin{align}
%     \widehat{M_{\mathrm{f}}} :=1/\sqrt{\wmin} M_{\mathrm{f}}\leq 3\sqrt{m\beta}M_{\mathrm{f}}/\sqrt{\muglobal}\label{eq:self_concordant_param_of_sum}
% \end{align}
% self-concordant. Then, from Lemma~\ref{lemma:self_con_consequences}, by properties of self-concordant functions, for every $\x \in \reals^n$ we have
% \begin{align*}
%       \inner{\nabla f_{\w_k}(\x_k)}{\x_k-\x } \geq f_{\w_k}(\x_k) -f_{\w_k}(\x) + \frac{1}{\widehat{M_{\mathrm{f}}}^2} \omega\brac{\widehat{M_{\mathrm{f}}}\enorm{\x - \x_k}_{\x_k,\w_k} },
% \end{align*}
% Plugging this inequality into Eq.~\eqref{eq:camoo_gd_recursion} implies that
% \begin{align}
%     \enorm{\x_{k+1}-\x}^2 &\leq \enorm{\x_k-\x}^2 - 2\eta\brac{f_{\w_k}(\x_k) -f_{\w_k}(\x) + \frac{1}{\widehat{M_{\mathrm{f}}}^2} \omega\brac{ \widehat{M_{\mathrm{f}} } \enorm{\x - \x_k}_{\x_k,\w_k} }} + \eta^2\enorm{\nabla f_{\w_k}(\x_k)}^2. \label{eq:camoo_dist_from_x}
% \end{align}
% Recall that $\x_\star \in \argmin_{\x} f_i(\x)$ for every $i \in [m]$. Since $f_{\w_k}$ is $\beta$-smooth, by using Lemma~\ref{lemma:smooth-gradient-norm}, and plugging in $\x_\star$ we have
% \begin{align*}
%     \enorm{\x_{k+1}-\x_\star}^2 &\leq \enorm{\x_k-\x_\star}^2 - 2\eta\brac{f_{\w_k}(\x_k) -f_{\w_k}(\x_\star) + \frac{1}{\widehat{M_{\mathrm{f}}}^2} \omega\brac{\widehat{M_{\mathrm{f}}}\enorm{\x_\star - \x_k}_{\x_k,\w_k} }} + 2 \beta \eta^2 \brac{f_{\w_k}(\x_k) -f_{\w_k}(\x_\star)} \\
%     & =  \enorm{\x_k-\x_\star}^2 - 2\eta \frac{1}{\widehat{M_{\mathrm{f}}}^2} \omega\brac{\widehat{M_{\mathrm{f}}}\enorm{\x_\star - \x_k}_{\x_k,\w_k} } + 2\eta (\beta \eta - 1) \brac{f_{\w_k}(\x_k) -f_{\w_k}(\x_\star)}.
% \end{align*}
% By using Lemma~\ref{lemma:optimality_of_x_star} it holds that $f_{\w_k}(\x_k) -f_{\w_k}(\x_\star)\geq 0$, and since $0 < \eta \leq 1/2\beta$, it holds that $2\eta (\beta \eta - 1) \brac{f_{\w_k}(\x_k) -f_{\w_k}(\x_\star)} \leq 0$. Then, by using the lower bound from Lemma~\ref{lemma:self_con_consequences}, i.e. $\omega\brac{t} \geq \frac{t^2}{2\brac{1+t}}$, the following holds
% \begin{align*}
%     \enorm{\x_{k+1}-\x_\star}^2 &\leq \enorm{\x_k-\x_\star}^2 -2\eta \frac{\enorm{\x_\star - \x_k}_{\x_k,\w_k}^2}{1+\widehat{M_{\mathrm{f}}}\enorm{\x_\star - \x_k}_{\x,\w_k}}.
% \end{align*}
% Note that $\lambda_{\min}\brac{\nabla^2 f_{\w_k}(\x_k)} \enorm{\x_\star - \x_k}^2 \leq \enorm{\x_\star - \x_k}_{\x_k,\w_k}^2 \leq \lambda_{\max}\brac{\nabla^2 f_{\w_k}(\x_k)} \enorm{\x_\star - \x_k}^2$. By using the following: $\lambda_{\min}\brac{\nabla^2 f_{\w_k}(\x_k)} \geq (3/4)\muglobal$ (Eq.~\eqref{eq:strongly_convex_param_of_AMOOO}), $\lambda_{\max}\brac{\nabla^2 f_{\w_k}(\x_k)} \leq \beta$ (smoothness), $\widehat{M_{\mathrm{f}}} \leq 3\sqrt{m\beta}M_{\mathrm{f}} /\sqrt{\muglobal}$ (Eq.~\eqref{eq:self_concordant_param_of_sum}), and $\eta = 1/2\beta$, we obtain
% \begin{align*}
%     \enorm{\x_{k+1}-\x_\star}^2 &\leq \enorm{\x_k-\x_\star}^2 -\frac{3 \muglobal}{4 \beta} \frac{\enorm{\x_\star - \x_k}^2}{1+\brac{3\sqrt{m}\beta M_{\mathrm{f}}/\sqrt{\muglobal}}\enorm{\x_\star - \x_k}}.
% \end{align*}
% Now, we are ready for the last step. Denote $\alpha_1 = \frac{3\muglobal}{4\beta}$, and $\alpha_2 = \frac{3\sqrt{m}\beta M_{\mathrm{f}}}{\sqrt{\muglobal}}$. Since $\alpha_1 \in (0,1]$, $\alpha_2 \in \reals_+$, and $\enorm{\x-\x_\star} \in \reals_+$ for every $\x \in \reals^n$, we arrive to the recurrence relation analyzed in Lemma~\ref{lemma:iteration_bound}. Then, we obtain
%     \begin{align*}
%         \enorm{\x_{k} - \x_\star} \leq 
%         \begin{cases}
%             \frac{\sqrt{\muglobal}}{3\sqrt{m}\beta M_{\mathrm{f}}} \brac{1-\frac{3\muglobal}{8\beta}}^{(k-k_0)/2}  & k\geq k_0\\
%             \enorm{\x_0 - \x_\star}- k \frac{\muglobal^{3/2}}{16 \beta^2 \sqrt{m} M_{\mathrm{f}}} & o.w.
%         \end{cases}
%     \end{align*}
% where $k_0 := \left\lceil \frac{16 \beta  \brac{\enorm{\x_0 - \x_\star} 3\sqrt{m}\beta M_{\mathrm{f}} -\sqrt{\muglobal}} }{ 3\muglobal^{3/2}}\right\rceil$.
% \end{proof}

% \subsection{Proof of Theorem~\ref{thm:exact_pamoo_convergence}}\label{app:pamoo}
 
% Let us restate the result:
% \ExactPAmooConvergence*

% \begin{proof}
% Recall that for every $\w\in \reals^m_+$ it holds that $f_{\w}$ is a convex function. Hence, for every $\x,\y \in \reals^n$ it holds that
% \begin{align*}
%     &f_{\w}(\x) - f_{\w}(\y)  \leq \nabla f_\w(\x)^T(\x-\y). 
% \end{align*}
% Recall that the step size $\eta = 1$, then the update rule is given by $\x_{k+1} = \x_k - \nabla f_{\w_k}(\x_k)$. Then, by using the previous equation, for every $\x \in \reals^n$ we have
% \begin{align}
%     \enorm{\x_{k+1}-\x}^2 &=\enorm{\x_k-\x}^2 - 2\inner{\nabla f_{\w_k}(\x_k)}{\x_k - \x} + \enorm{\nabla f_{\w_k}(\x_k)}^2 \nonumber\\
%     &\leq \enorm{\x_k-\x}^2 - 2 \brac{f_{\w_k}(\x_k)- f_{\w_k} (\x)} +\enorm{\nabla f_{\w_k}(\x_k)}^2 , \label{eq:PAMOO_dist_from_x}
% \end{align}
% Recall that $\x_\star \in \argmin_{\x \in \reals^n} f_i(\x)$ for every $i \in [m]$. Since the update rule of \texttt{PAMOO} is 
% $$
% \w_k\in \argmax_{\w\in \reals^m_+} 2\brac{f_{\w_k}(\x_k)- f_{\w_k} (\x_\star)} - \enorm{\nabla f_{\w_k}(\x_k)}^2,
% $$
% the following holds
% \begin{align}
%     \enorm{\x_{k+1}-\x_\star}^2 &\leq \enorm{\x_k-\x_\star}^2 -  \max_{\w \in \reals_+^m} \Big{\{} 2\brac{f_{\w}(\x_k)- f_{\w} (\x_\star)} - \enorm{\nabla f_{\w}(\x_k)}^2 \Big{\}}, \label{eq:PAMOO_dist_from_opt}
% \end{align}
% Denote $\w_\star = \argmax\limits_{\w\in \Delta_{m,\wmin}} \lambda_{\min}\brac{\sum_{i=1}^m w_i \nabla^2 f_i(\x_\star)}$, $a_k = f_{\w_\star}(\x_k)- f_{\w_\star} (\x_\star)$, and $b_k = \enorm{\nabla f_{\w_\star}(\x_k)}^2$. Let $w(\x_k) = \w_\star \frac{a_k}{b_k} \in \reals^m_+$, we can lower bound of the last expression as follows
% \begin{align*}
%     \max_{\w\in \reals_+^m} \left[ 2\brac{f_{\w}(\x_k)- f_{\w} (\x_\star)} - \enorm{\nabla f_{\w}(\x_k)}^2 \right] & \geq 2\brac{f_{\w(\x_k)}(\x_k)- f_{\w(\x_k)} (\x_\star)}  -\enorm{\nabla f_{\w(\x_k)}(\x_k)}^2 \\
%     & =   \frac{\brac{f_{\w_\star}(\x_k)- f_{\w_\star} (\x_\star)}^2}{\enorm{\nabla f_{\w_\star}(\x_k)}^2}.
% \end{align*}
% Since $\w_\star\in \Delta_{m,\wmin}$ it holds that $f_{\w_\star}$ is $\beta$ smooth. Then, it holds that $\enorm{\nabla f_{\w_\star}(\x)}^2 \leq 2\beta \brac{f_{\w_\star}(\x)- f_{\w_\star} (\x_\star)}$ for every $\x$, and we have
% \begin{align*}
%      \max_{\w\in \reals_+^m} \left[ 2\brac{f_{\w}(\x_k)- f_{\w} (\x_\star)} - \enorm{\nabla f_{\w}(\x_k)}^2 \right] & \geq \frac{f_{\w_\star}(\x_k)- f_{\w_\star} (\x_\star)}{2 \beta} 
% \end{align*}
% Plugging this in Eq.~\eqref{eq:PAMOO_dist_from_opt}, we arrive to 
% \begin{align*}
%     \enorm{\x_{k+1}-\x_\star}^2 &\leq \enorm{\x_k-\x_\star}^2 -  \frac{ f_{\w_\star}(\x_k)- f_{\w_\star} (\x_\star)}{2 \beta}
% \end{align*}
% By Lemma~\ref{lemma:self_concordant} it holds that $f_{\w_\star}$ is $\widehat{M_{\mathrm{f}}}:=1/\sqrt{\wmin} M_{\mathrm{f}}$ self concordant. Then, From Lemma~\ref{lemma:self_con_consequences}, and its lower bound , i.e. $\omega\brac{t} \geq \frac{t^2}{2\brac{1+t}}$, we have
% \begin{align*}
%        f_{\w_\star}(\x_k) -f_{\w_\star}(\x_\star) \geq \inner{\nabla f_{\w_\star}(\x_\star)}{\x_k - \x_\star} +  \frac{\enorm{\x_k - \x_\star}_{ \x_\star,\w_\star}^2}{2\brac{1+\widehat{M_{\mathrm{f}}}\enorm{\x_k - \x_\star}_{\x_\star,\w_\star}}} = \frac{\enorm{\x_k - \x_\star}_{ \x_\star,\w_\star}^2}{2\brac{1+\widehat{M_{\mathrm{f}}}\enorm{\x_k - \x_\star}_{\x_\star,\w_\star}}}.
% \end{align*}
% The equality is due to the optimality condition, $\nabla f_i(\x_\star)=0$ for every $i \in [m]$, thus, $\nabla f_{\w_\star}(\x_\star) = \bold{0}$.
% Combining the last two equations, we have 
% \begin{align*}
%     \enorm{\x_{k+1}-\x_\star}^2 &\leq \enorm{\x_k-\x_\star}^2 -  \frac{1}{4 \beta} \frac{\enorm{\x_k - \x_\star}_{ \x_\star,\w_\star}^2}{1+\widehat{M_{\mathrm{f}}}\enorm{\x_k - \x_\star}_{\x_\star,\w_\star}}
% \end{align*}
% Note that $\lambda_{\min}\brac{\nabla^2 f_{\w_\star}(\x_\star)} \enorm{\x_\star - \x_k}^2 \leq \enorm{\x_\star - \x_k}_{\x_\star,\w_\star}^2 \leq \lambda_{\max}\brac{\nabla^2 f_{\w_\star}(\x_\star)} \enorm{\x_\star - \x_k}^2$. Since $\lambda_{\max}\brac{\nabla^2 f_{\w_\star}(\x_\star)} \leq \beta$ (smoothness), and since $w_{\min}= \mulocal /(8m\beta)$, then $\widehat{M_{\mathrm{f}}} \leq 3\sqrt{m\beta}M_{\mathrm{f}} /\sqrt{\mulocal}$. Thus, it holds that
% \begin{align*}
%     \enorm{\x_{k+1}-\x_\star}^2 &\leq \enorm{\x_k-\x_\star}^2 -  \frac{1}{4 \beta} \frac{\lambda_{\min}\brac{\nabla^2 f_{\w_\star}(\x_\star)} \enorm{\x_\star - \x_k}^2}{1+ \frac{3\sqrt{m} M_{\mathrm{f}} \beta}{\sqrt{\mulocal}}  \enorm{\x_k - \x_\star}}
% \end{align*}
% Using the assumption that $\max\limits_{\w\in \Delta_m}\lambda_{\min}\brac{\nabla^2 f_{\w}(\x_\star)} \geq \mulocal$, Lemma~\ref{lemma:mu_star_minimal_eigenvalue}, we have that
% \begin{align*}
%     \lambda_{\min} \brac{\nabla^2f_{\w_\star}(\x_\star)}\geq \max\limits_{\w\in \Delta_m}\lambda_{\min}\brac{\nabla^2 f_{\w}(\x_\star)} - 2m\wmin\beta \geq \mulocal - \mulocal/4 = (3/4)\mulocal.
% \end{align*}
% Finally, we obtain the recurring equation we wish:
% \begin{align*}
%     \enorm{\x_{k+1}-\x_\star}^2 &\leq \enorm{\x_k-\x_\star}^2 -  \frac{3 \mulocal}{16 \beta} \frac{ \enorm{\x_\star - \x_k}^2}{1+ \frac{3\sqrt{m} M_{\mathrm{f}} \beta}{\sqrt{\mulocal}}  \enorm{\x_k - \x_\star}}
% \end{align*} 
% Denote $\alpha_1 = \frac{3\mulocal}{16\beta}$, and $\alpha_2 = \frac{3\sqrt{m}\beta M_{\mathrm{f}}}{\sqrt{\mulocal}}$. Note that $\alpha_1 \in (0,1]$, $\alpha_2 \in \reals_+$, and $\enorm{\x-\x_\star} \in \reals_+$ for every $\x \in \reals^n$, we arrive to the recurrence relation analyzed in Lemma~\ref{lemma:iteration_bound}. Then, we obtain
% \begin{align*}
%     \enorm{\x_{k} - \x_\star} \leq 
%     \begin{cases}
%         \frac{\sqrt{\mulocal}}{3\sqrt{m}\beta M_{\mathrm{f}}} \brac{1-\frac{3\mulocal}{32\beta}}^{(k-k_0)/2}  & k\geq k_0\\
%         \enorm{\x_0 - \x_\star}- k \frac{\mulocal^{3/2}}{64 \beta^2 \sqrt{m} M_{\mathrm{f}}} & o.w.
%     \end{cases}
% \end{align*}
% where $k_0 := \left\lceil \frac{64 \beta  \brac{\enorm{\x_0 - \x_\star} 3\sqrt{m}\beta M_{\mathrm{f}} -\sqrt{\mulocal}} }{ 3\mulocal^{3/2}}\right\rceil$.
% \end{proof}


% \subsection{Proof of Proposition~\ref{thm:app_hessian}}\label{app:weyls consequence}
% The proof of Proposition~\ref{thm:app_hessian} is a corollary of Theorem~\ref{thm:weyls} (Weyl's Theorem). We establish the result for a general deviation in Hessian matrices without requiring it to be necessarily diagonal.

% Let us restate the result:
% \ApproxHessian*

% \begin{proof}
    
% Denote $\A_i := \nabla^2 f_i(\x) + \Delta_i$ for every $i\in [m]$, and $\sum_i^m \Delta_i = \Delta$. Let $\w_\star $, and $\hat{\w}_\star$ denote the solution of,
%     \begin{align*}
%         \w_\star \in \argmax_{\w\in \Delta} \lambda_{\min}\brac{\sum_i w_i \nabla^2 f_i(\x)}, ~~~~~ \text{and} ~~~~~~~ \hat{\w}_\star \in \argmax_{\w\in \Delta} \lambda_{\min}\brac{\sum_i w_i \A_i},
%     \end{align*}
%     respectively. Let $g(\w_\star)$, and $\hat{g}(\hat{\w}_\star)$ denote the optimal value, $g(\w_\star) = \lambda_{\min} \brac{\sum_i w_{\star, i}  \nabla^2 f_i(\x)}$, and $\hat{g}(\hat{\w}_\star) = \lambda_{\min} \brac{\sum_i \hat{w}_{\star, i} \A_i}$. Then, since $\hat{g}(\w_\star) -\hat{g}(\hat{\w}_\star)\leq 0$ by the optimality of $\hat{\w}_\star$ on $\hat{g}$, the following holds
%     \begin{align*}
%         g(\w_\star) & = g(\w_\star) - \hat{g}(\w_\star) + \hat{g}(\w_\star) -\hat{g}(\hat{\w}_\star) +\hat{g}(\hat{\w}_\star) - g(\hat{\w}_\star) +g(\hat{\w}_\star) \\
%         & \leq |g(\w_\star) - \hat{g}(\w_\star)|  + |\hat{g}(\hat{\w}_\star) - g(\hat{\w}_\star)| +g(\hat{\w}_\star)\\
%     \end{align*}
%     Using Theorem~\ref{thm:weyls} (Weyl's Theorem) the followings are hold: $|g(\w_\star) - \hat{g}(\w_\star)| \leq \Delta$, and $|\hat{g}(\hat{\w}_\star) - g(\hat{\w}_\star)| \leq \Delta$. Then, we obtain 
%     \begin{align*}
%         g(\w_\star) & \leq 2\enorm{\Delta} +g(\hat{\w}_\star)
%     \end{align*}
%     Finally, since $g(\w_\star)\geq \muglobal$, by Definition~\ref{def:mu_global}, we obtain the proof.
% \end{proof}
